# Supplementary material for: Advances in Electron Microscopy with Deep Learning
Source: arXiv:2101.01178 source file (2021-03-11)
Supplement: Supplementary file 1 [file paper_adaptive_scans_supplementary.pdf]

# Supplementary Information: Adaptive Partial Scanning Transmission Electron Microscopy with Reinforcement Learning

Jeffrey M. Ede<sup>1,a</sup>

<sup>1</sup>University of Warwick, Department of Physics, Coventry, CV4 7AL, UK

<sup>a</sup>j.m.ede@warwick.ac.uk

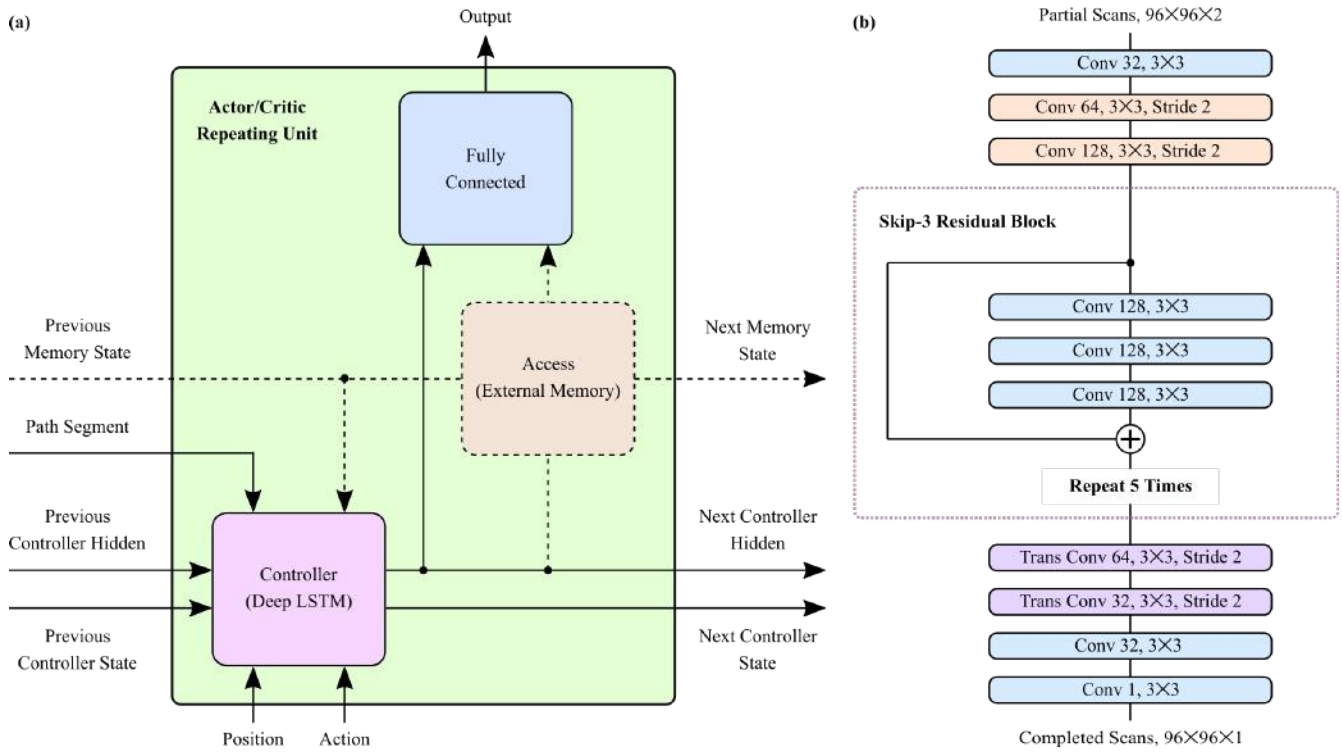

**Figure S1.** Actor, critic and generator architecture. a) An actor outputs action vectors whereas a critic predicts losses. Dashed lines are for extra components in a DNC. b) A convolutional generator completes partial scans.

## S1 Detailed Architecture

Detailed actor, critic and generator architecture is shown in figure S1. Actors and critics have almost identical architecture, except actor fully connected layers output action vectors whereas critic fully connected layers output predicted losses. In most of our experiments, actors and critics are deep LSTMs<sup>1</sup>. However, we also augment deep LSTMs with dynamic external memory to create DNCs<sup>2</sup> in some of our experiments. Configuration details of actor and critic components shown in figure S1(a) follow.

**Controller (Deep LSTM):** A two-layer deep LSTM with 256 hidden units in each layer. To reduce signal attenuation, we add skip connections from inputs to the second LSTM layer and from the first LSTM layer to outputs. Weights are initialized from truncated normal distributions and biases are zero initialized. In addition, we add a bias of 1 to the forget gate to reduce forgetting at the start of training<sup>3</sup>. Initial LSTM cell and hidden states are initialized with trainable variables<sup>4</sup>.

**Access (External Memory):** Our DNC implementation is adapted from Google Deepmind's<sup>2,5</sup>. We use 4 read heads and 1

write head to control access to dynamic external memory, which has 16 slots with a word size of 64.

**Fully Connected:** A dense layer linearly connects inputs to outputs. Weights are initialized from a truncated normal distribution and there are no biases.

**Conv  $d, wxw$ , Stride,  $x$ :** Convolutional layer with a square kernel of width,  $w$ , that outputs  $d$  feature channels. If the stride is specified, convolutions are only applied to every  $x$ th spatial element of their input, rather than to every element. Striding is not applied depthwise.

**Trans Conv  $d, wxw$ , Stride,  $x$ :** Transpositional convolutional layer with a square kernel of width,  $w$ , that outputs  $d$  feature channels. If the stride is specified, convolutions are only applied to every  $x$ th spatial element of their input, rather than to every element. Striding is not applied depthwise.

⊕: Circled plus signs indicate residual connections where incoming tensors are added together. Residuals help reduce signal attenuation and allow a network to learn perturbative transformations more easily.

The actor and critic cooperate with a convolutional generator, shown in figure S1(b), to complete partial scans. Our generator is constructed from convolutional layers<sup>6</sup> and skip-3 residual blocks<sup>7</sup>. Each convolutional layer is followed by ReLU<sup>8</sup> activation then batch normalization<sup>9</sup>, and residual connections are added between activation and batch normalization. The convolutional weights are Xavier<sup>10</sup> initialized and biases are zero initialized.

## S2 Additional Regularization

We apply L2 regularization<sup>11</sup> to decay generator parameters by a factor,  $\beta = 0.99999$ , at each training iteration. This decay rate is heuristic and the L2 regularization is primarily a precaution against overfitting. Further, adding L2 regularization did not have a noticeable effect on performance. We also investigated gradient clipping<sup>12–15</sup> to a range of static and dynamic thresholds for actor and critic training. However, we found that gradient clipping decreases convergence if clipping thresholds are too small and otherwise does not have a noticeable effect.

## S3 Additional Experiments

This section present additional learning curves for architecture and learning policy experiments in figure S2. For example, learning curves in figure S2(a) show that generator training with an exponentially decayed cyclic learning rate<sup>16</sup> results in faster convergence and lower final errors than just using an exponentially decayed learning rate. We were concerned that a cyclic learning rate might cause generator loss oscillations if the learning rate oscillated too high. Indeed, our investigation of loss normalization was, in part, to prevent potential generator loss oscillations from destabilizing critic training. However, our learning policy results in generator losses that steadily decay throughout training.

To train actors by BPTT, we differentiate losses predicted by critics w.r.t. actor parameters by the chain rule,

$$\Delta\theta = \frac{1}{NT} \sum_i^N \sum_t^T \frac{\partial Q(h_t^i, a_t^i)}{\partial \theta} = \frac{1}{NT} \sum_i^N \sum_t^T \frac{\partial Q(h_t^i, a_t^i)}{\partial \mu(h_t^i)} \frac{\partial \mu(h_t^i)}{\partial \theta}. \quad (\text{S1})$$

An alternative approach is to replace  $\partial Q(h_t^i, a_t^i)/\partial \mu(h_t^i)$  with a derivative w.r.t. replayed actions,  $\partial Q(h_t^i, a_t^i)/\partial a_t^i$ . This is equivalent to adding noise,  $\text{stop\_gradient}(a_t^i - \mu(h_t^i))$ , to an actor action,  $\mu(h_t^i)$ , where  $\text{stop\_gradient}(x)$  is a function that stops gradient backpropagation to  $x$ . However, learning curves in figure S2(b) show that differentiation w.r.t. live actor actions results in faster convergence to lower losses. Results for  $\partial Q(h_t^i, a_t^i)/\partial a_t^i$  are similar if OU exploration noise is doubled.

Most STEM signals are imaged at several times their Nyquist rates<sup>17</sup>. To investigate adaptive STEM performance on signals imaged close to their Nyquist rates, we downsampled STEM images to  $96 \times 96$ . Learning curves in figure S2(c) show that losses are lower for oversampled STEM crops. Following, we investigated if MSEs vary for training with different loss metrics by adding a Sobel loss,  $\lambda_S L_S$ , to generator losses. Our Sobel loss is

$$L_S = \text{MSE}(S(G(s)), S(I_N)), \quad (\text{S2})$$

where  $S(x)$  computes a channelwise concatenation of horizontal and vertical Sobel derivatives<sup>18</sup> of  $x$ , and we chose  $\lambda_S = 0.1$  to weight the contribution of  $L_S$  to the total generator loss,  $L_G + \lambda_S L_S$ . Learning curves in figure S2(c) show that Sobel losses do not decrease training MSEs for STEM crops. However, Sobel losses decrease MSEs for downsampled STEM images. This motivates the exploration of alternative loss functions<sup>19</sup> to further improve performance. For example, our earlier work shows that generator training as part of a generative adversarial network<sup>20–23</sup> (GAN) can improve STEM image realism<sup>24</sup>. Similarly, we expect that generated image realism could be improved by training generators with perceptual losses<sup>25</sup>.

After we found that adding a Sobel loss can decrease MSEs, we also experimented with other loss functions, such as the maximum MSE of  $5 \times 5$  regions. Learning curves in figure S2(d) show that MSEs result in faster convergence than maximum

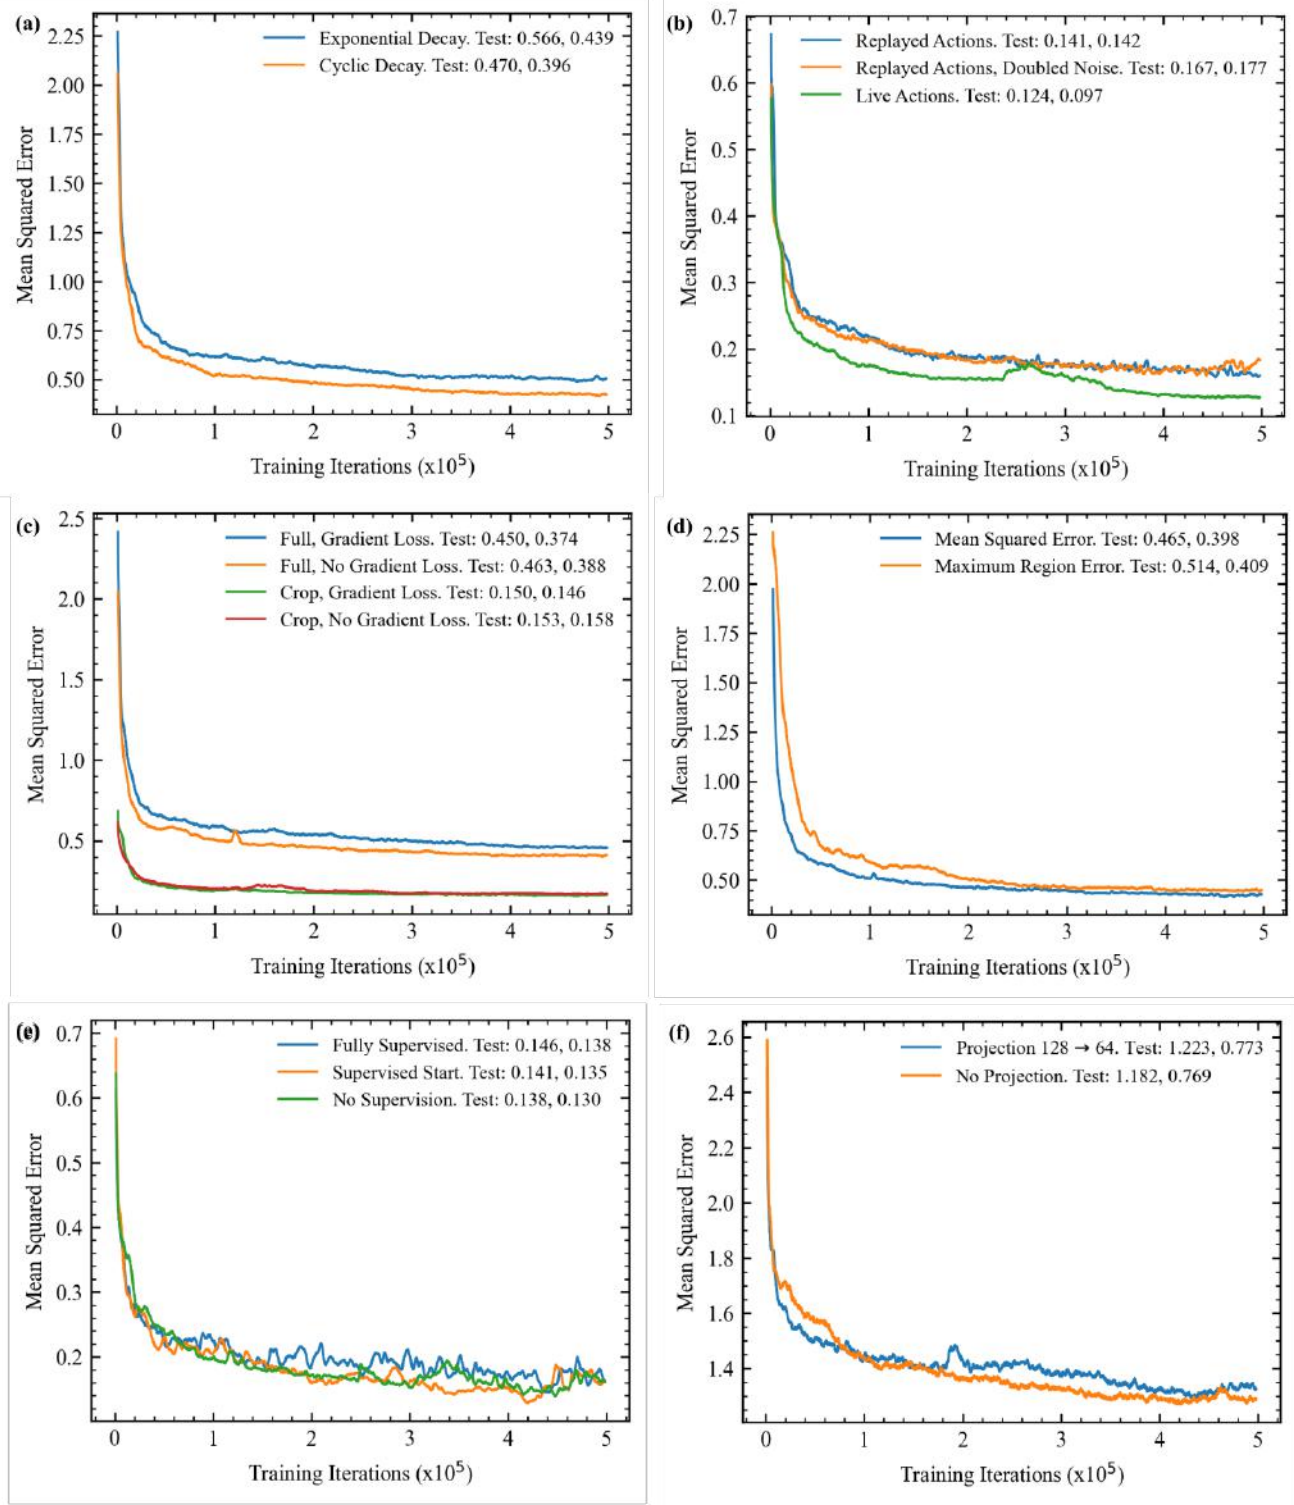

**Figure S2.** Learning curves for a) exponentially decayed and exponentially decayed cyclic learning rate schedules, b) actor training with differentiation w.r.t. live or replayed actions, c) images downsampled or cropped from full images to  $96 \times 96$  with and without additional Sobel losses, d) mean squared error and maximum regional mean squared error loss functions, e) supervision throughout training, supervision only at the start, and no supervision, and f) projection from 128 to 64 hidden units or no projection. All learning curves are 2500 iteration boxcar averaged, and results in different plots are not directly comparable due to varying experiment settings. Means and standard deviations of test set errors, “Test: Mean, Std Dev”, are at the ends of graph labels.

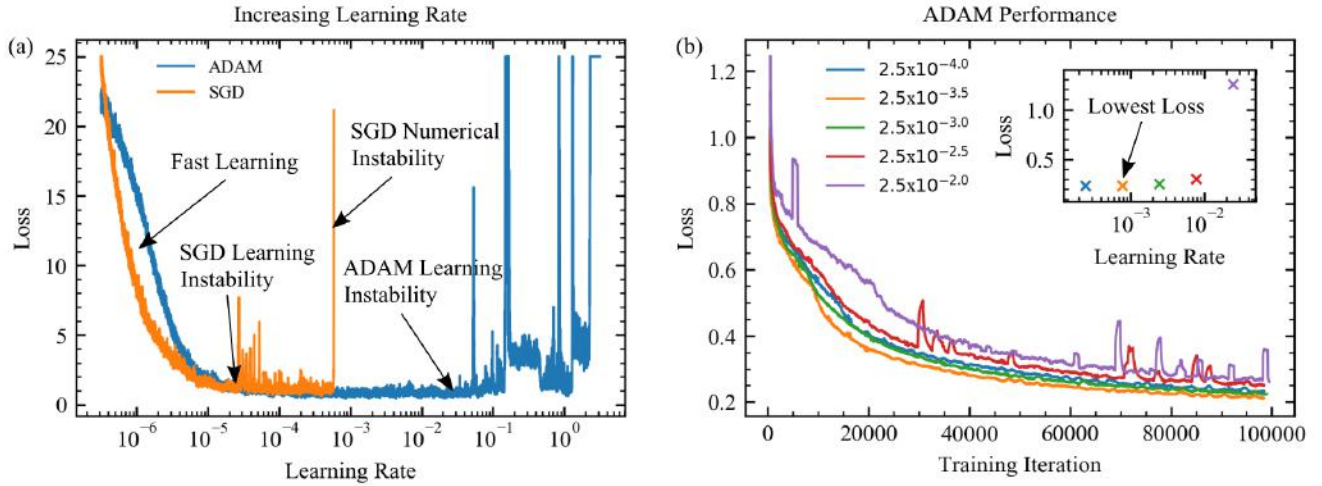

**Figure S3.** Learning rate optimization. a) Learning rates are increased from  $10^{-6.5}$  to  $10^{0.5}$  for ADAM and SGD optimization. At the start, convergence is fast for both optimizers. Learning with SGD becomes unstable at learning rates around  $2.2 \times 10^{-5}$ , and numerically unstable near  $5.8 \times 10^{-4}$ , whereas ADAM becomes unstable around  $2.5 \times 10^{-2}$ . b) Training with ADAM optimization for learning rates listed in the legend. Learning is visibly unstable at learning rates of  $2.5 \times 10^{-2.5}$  and  $2.5 \times 10^{-2}$ , and the lowest inset validation loss is for a learning rate of  $2.5 \times 10^{-3.5}$ . Learning curves in (b) are 1000 iteration boxcar averaged. Means and standard deviations of test set errors, “Test: Mean, Std Dev”, are at the ends of graph labels.

region losses; however, both loss functions result in similar final MSEs. We expect that MSEs calculated with every output pixel result in faster convergence than maximum region errors as more pixels inform gradient calculations. In any case, we expect that a better approach to minimize maximum errors is to use a higher order loss function, such as mean quartic errors. If training with a higher-order loss function is unstable, it might be stabilized by adaptive learning rate clipping<sup>26</sup>.

Target losses can be directly computed with Bellman’s equation, rather than with target networks. We refer to such directly computed target losses as “supervised” losses,

$$Q_t^{\text{super}} = \sum_{t'=t}^T \gamma^{t'-t} L_{t'}, \quad (\text{S3})$$

where where  $\gamma \in [0, 1)$  discounts future step losses,  $L_t$ . Learning curves for full supervision, supervision linearly decayed to zero in the first  $10^5$  iterations, and no supervision are shown in figure S2(e). Overall, final errors are similar for training with and without supervision. However, we find that learning is usually more stable without supervised losses. As a result, we do not recommend using supervised losses.

To accelerate convergence and decrease computation, an LSTM with  $n_h$  hidden units can be augmented by a linear projection layer with  $n_p < 3n_h/4$  units<sup>27</sup>. Learning curves in figure S2(f) are for  $n_h = 128$  and compare training with a projection to  $n_p = 64$  units and no projection. Adding a projecting layer increases the initial rate of convergence; however, it also increases final losses. Further, we found that training becomes increasingly prone to instability as  $n_p$  is decreased. As a result, we do not use projection layers in our actor or critic networks.

Generator learning rate optimization is shown in figure S3. To find the best initial learning rate for ADAM optimization, we increased the learning rate until training became unstable, as shown in figure S3(a). We performed the learning rate sweep over  $10^4$  iterations to avoid results being complicated by losses rapidly decreasing in the first couple of thousand. The best learning rate was then selected by training for  $10^5$  iterations with learning rates within a factor of 10 from a learning rate  $10\times$  lower than where training became unstable, as shown in figure S3(b). We performed initial learning rate sweeps in figure S3(a) for both ADAM and stochastic gradient descent<sup>28</sup> (SGD) optimization. We chose ADAM as it is less sensitive to hyperparameter choices than SGD and because ADAM is recommended in the RDPG paper<sup>29</sup>.

## S4 Test Set Errors

Test set errors are computed for 3954 test set images. Most test set errors are similar to or slightly higher than training set errors. However, training with fixed paths, which is shown in figure 3(a) of the main article, results in high divergence of test and training set errors. We attribute this divergence to the generator overfitting to complete large regions that are not covered by

fixed scan paths. In comparison, our learning policy was optimized for training with a variety of adaptive scan paths where overfitting is minimal. After all  $10^6$  training iterations, means and standard deviations (mean, std dev) of test set errors for fixed paths 2, 3 and 4 are (0.170, 0.182), (0.135, 0.133), and (0.171, 0.184). Instead, we report lower test set errors of (0.106, 0.090), (0.073, 0.045), and (0.106, 0.090), respectively, at  $5 \times 10^5$  training iterations, which correspond to early stopping<sup>30,31</sup>. All other test set errors were computed after final training iterations.

## S5 Distortion Correction

A limitation of partial STEM is that images are usually distorted by probing position errors, which vary with scan path shape<sup>32</sup>. Distortions in raster scans can be corrected by comparing series of images<sup>33,34</sup>. However, distortion correction of adaptive scans is complicated by more complicated scan path shapes and microscope-specific actor command execution characteristics. We expect that command execution characteristics are almost static. Thus, it follows that there is a bijective mapping between probing locations in distorted adaptive partial scans and raster scans. Subsequently, we propose that distortions could be corrected by a cyclic generative adversarial network<sup>35</sup> (GAN). To be clear, this section outlines a possible starting point for future research that can be refined or improved upon. The method's main limitation is that the cyclic GAN would need to be trained or fine-tuned for individual scan systems.

Let  $I_{\text{partial}}$  and  $I_{\text{raster}}$  be unpaired partial scans and raster scans, respectively. A binary mask,  $M$ , can be constructed to be 1 at nominal probing positions in  $I_{\text{partial}}$  and 0 elsewhere. We introduce generators  $G_{p \rightarrow r}(I_{\text{partial}})$  and  $G_{r \rightarrow p}(I_{\text{raster}}, M)$  to map from partial scans to raster scans and from raster scans to partial scans, respectively. A mask must be input to the partial scan generator for it to output a partial scan with a realistic distortion field as distortions depend on scan path shape<sup>32</sup>. Finally, we introduce discriminators  $D_{\text{partial}}$  and  $D_{\text{raster}}$  are trained to distinguish between real and generated partial scans and raster scans, respectively, and predict losses that can be used to train generators to create realistic images. In short, partial scans could be mapped to raster scans by minimizing

$$L_{p \rightarrow r}^{\text{GAN}} = D_{\text{raster}}(G_{p \rightarrow r}(I_{\text{partial}})), \quad (\text{S4})$$

$$L_{r \rightarrow p}^{\text{GAN}} = D_{\text{partial}}(MG_{r \rightarrow p}(I_{\text{raster}}, M)), \quad (\text{S5})$$

$$L_{r \rightarrow p}^{\text{cycle}} = \text{MSE}(MG_{r \rightarrow p}(G_{p \rightarrow r}(I_{\text{partial}}), M), I_{\text{partial}}), \quad (\text{S6})$$

$$L_{p \rightarrow r}^{\text{cycle}} = \text{MSE}(G_{p \rightarrow r}(MG_{r \rightarrow p}(I_{\text{raster}}, M)), I_{\text{raster}}), \quad (\text{S7})$$

$$L_{p \rightarrow r} = L_{p \rightarrow r}^{\text{GAN}} + bL_{r \rightarrow p}^{\text{cycle}}, \quad (\text{S8})$$

$$L_{r \rightarrow p} = L_{r \rightarrow p}^{\text{GAN}} + bL_{p \rightarrow r}^{\text{cycle}}, \quad (\text{S9})$$

where  $L_{p \rightarrow r}$  and  $L_{r \rightarrow p}$  are total losses to optimize  $G_{p \rightarrow r}$  and  $G_{r \rightarrow p}$ , respectively. A scalar,  $b$ , balances adversarial and cycle-consistency losses.

## S6 Additional Examples

Additional sheets of test set adaptive scans are shown in figure S4 and figure S5. In addition, a sheet of test set spiral scans is shown in figure S6. Target outputs were low-pass filtered by a  $5 \times 5$  symmetric Gaussian kernel with a 2.5 px standard deviation to suppress high-frequency noise.

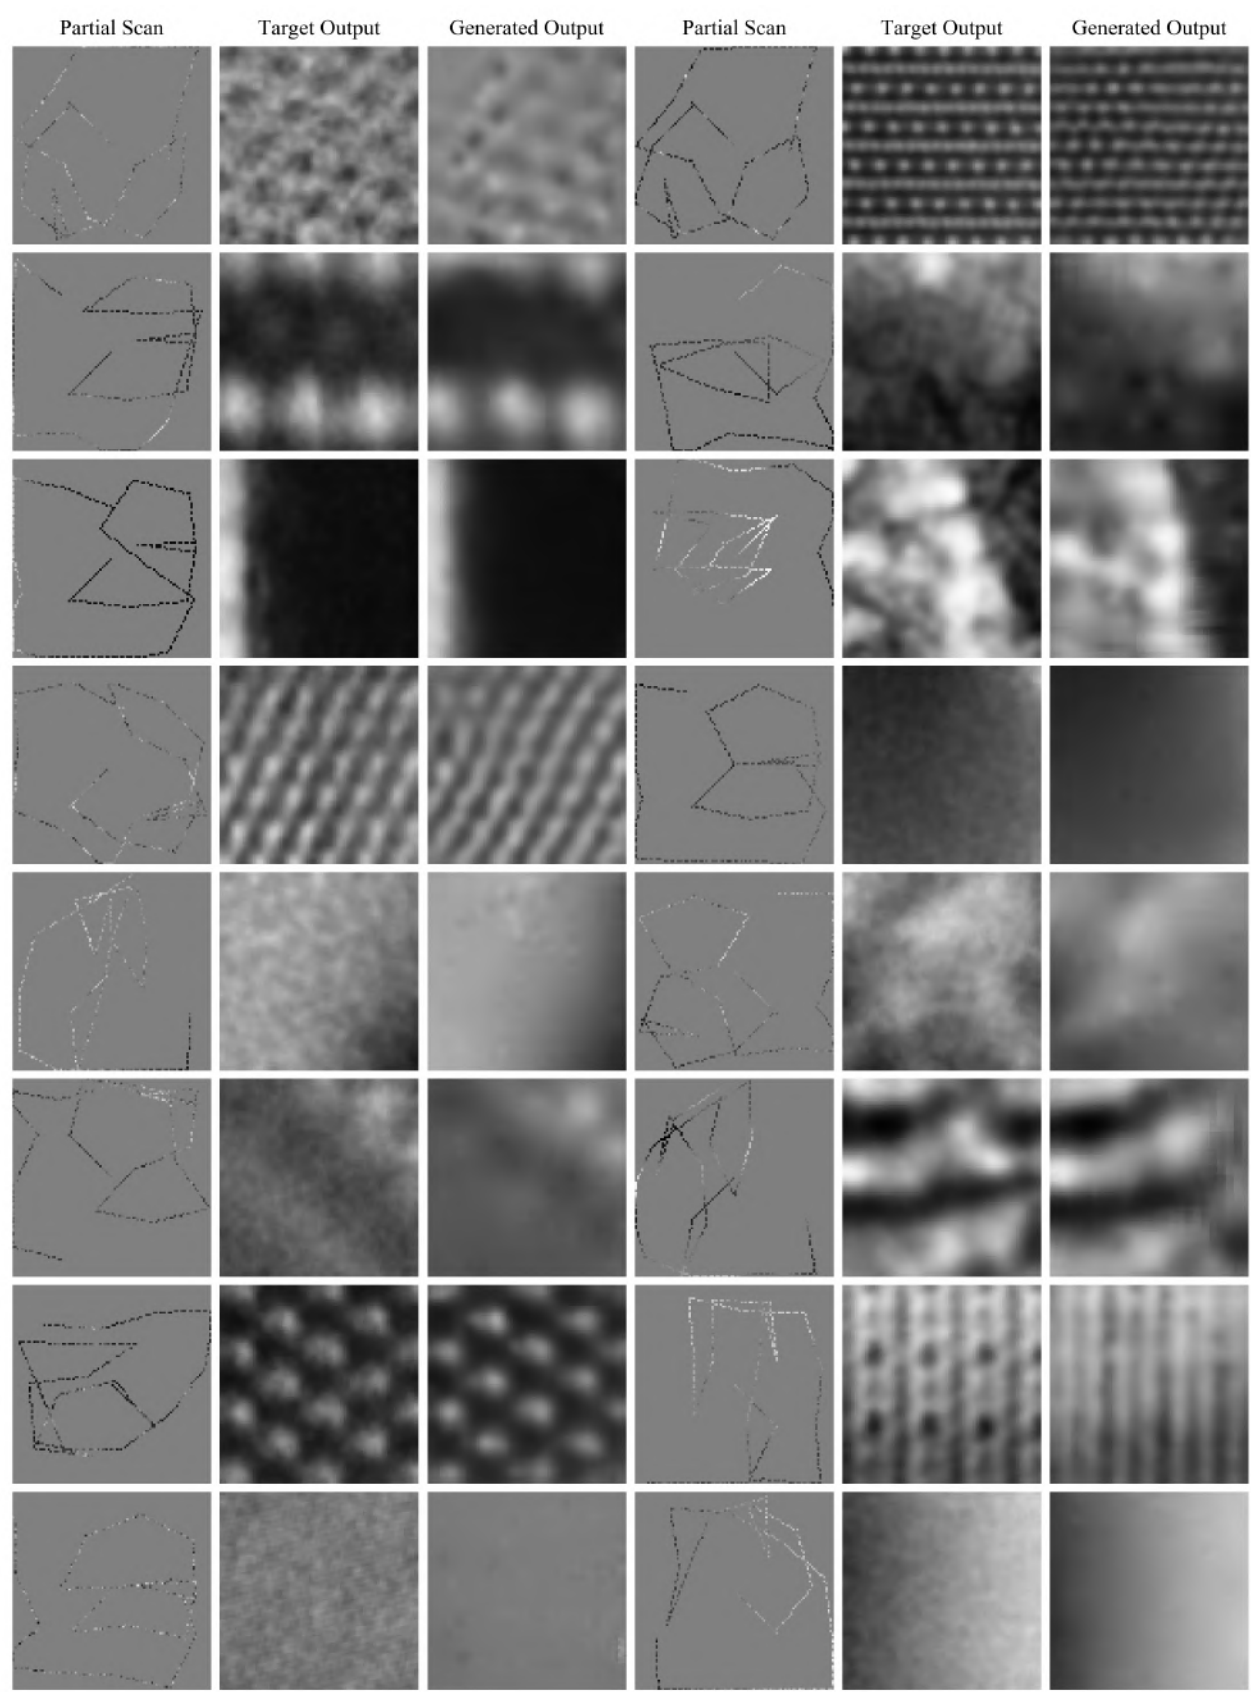

**Figure S4.** Test set 1/23.04 px coverage adaptive partial scans, target outputs, and generated partial scan completions for  $96 \times 96$  crops from STEM images.

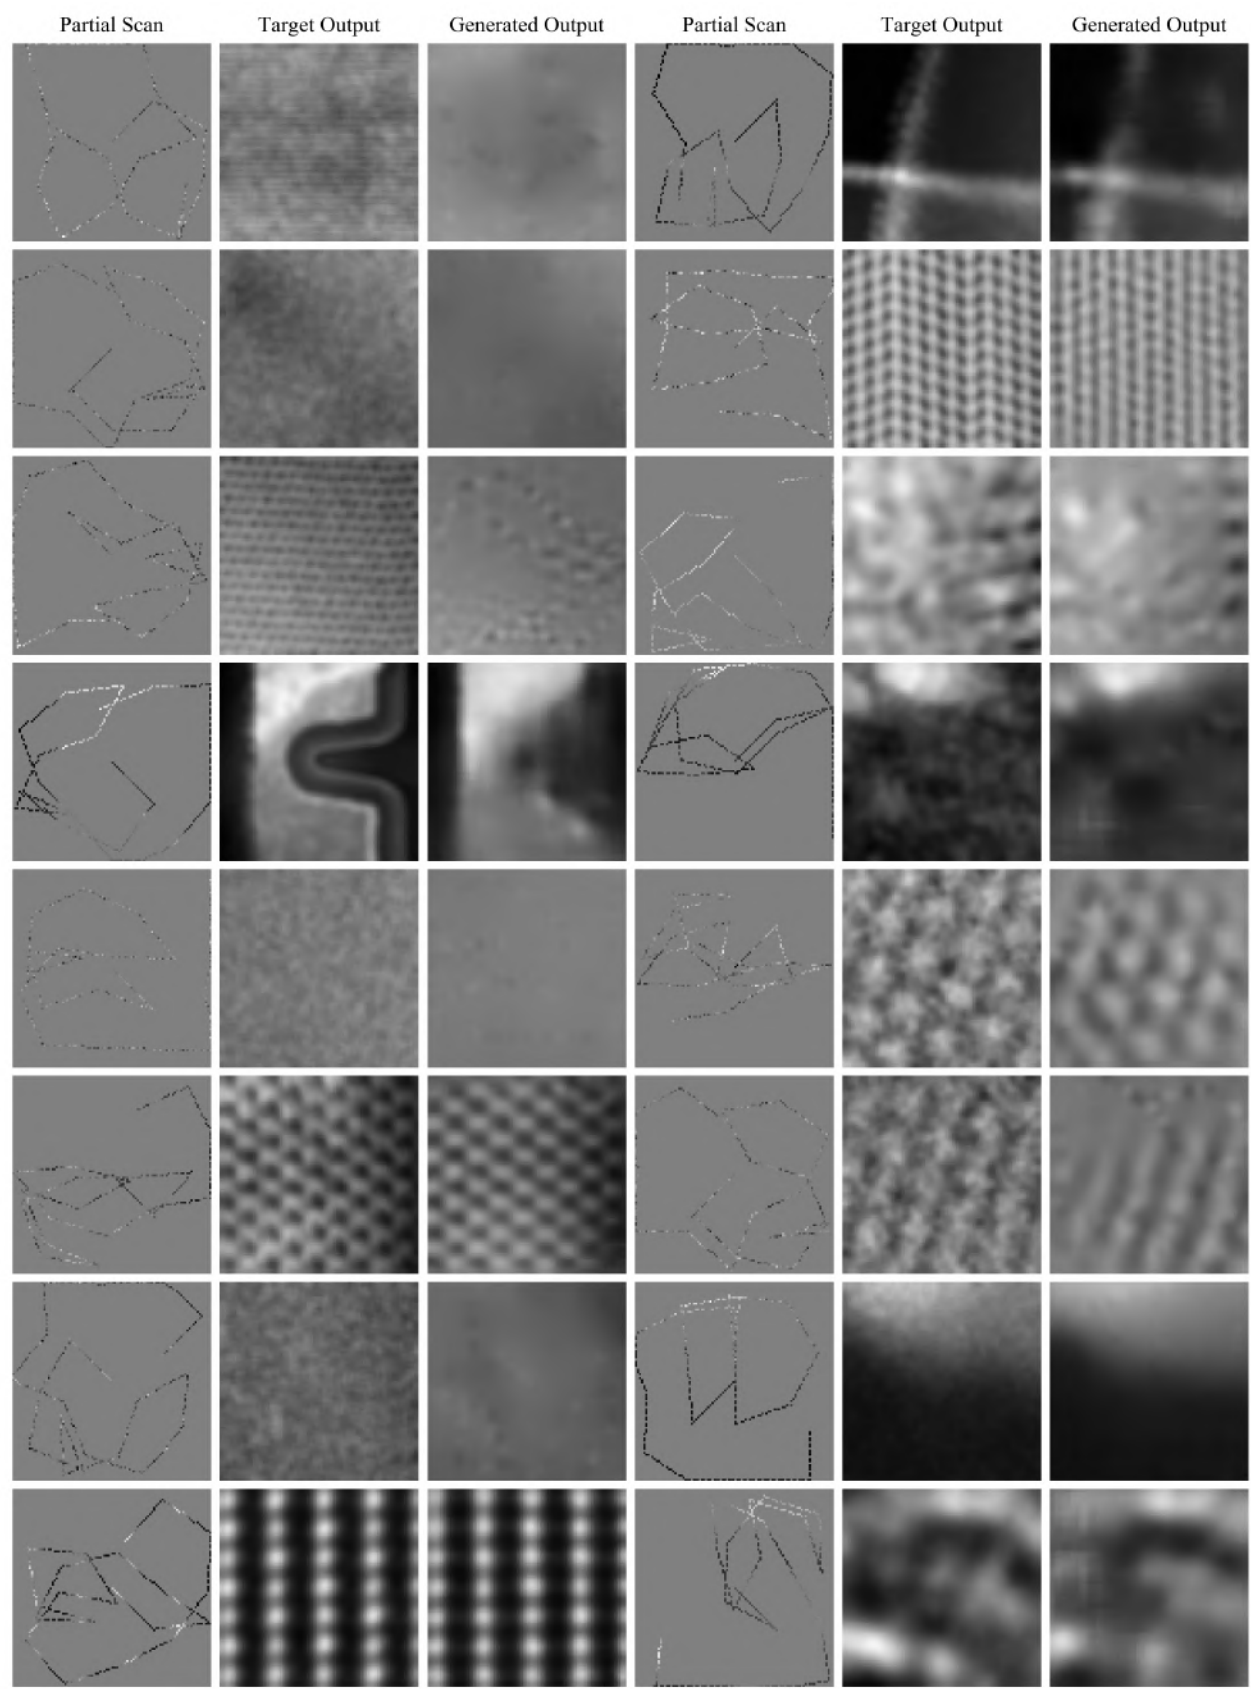

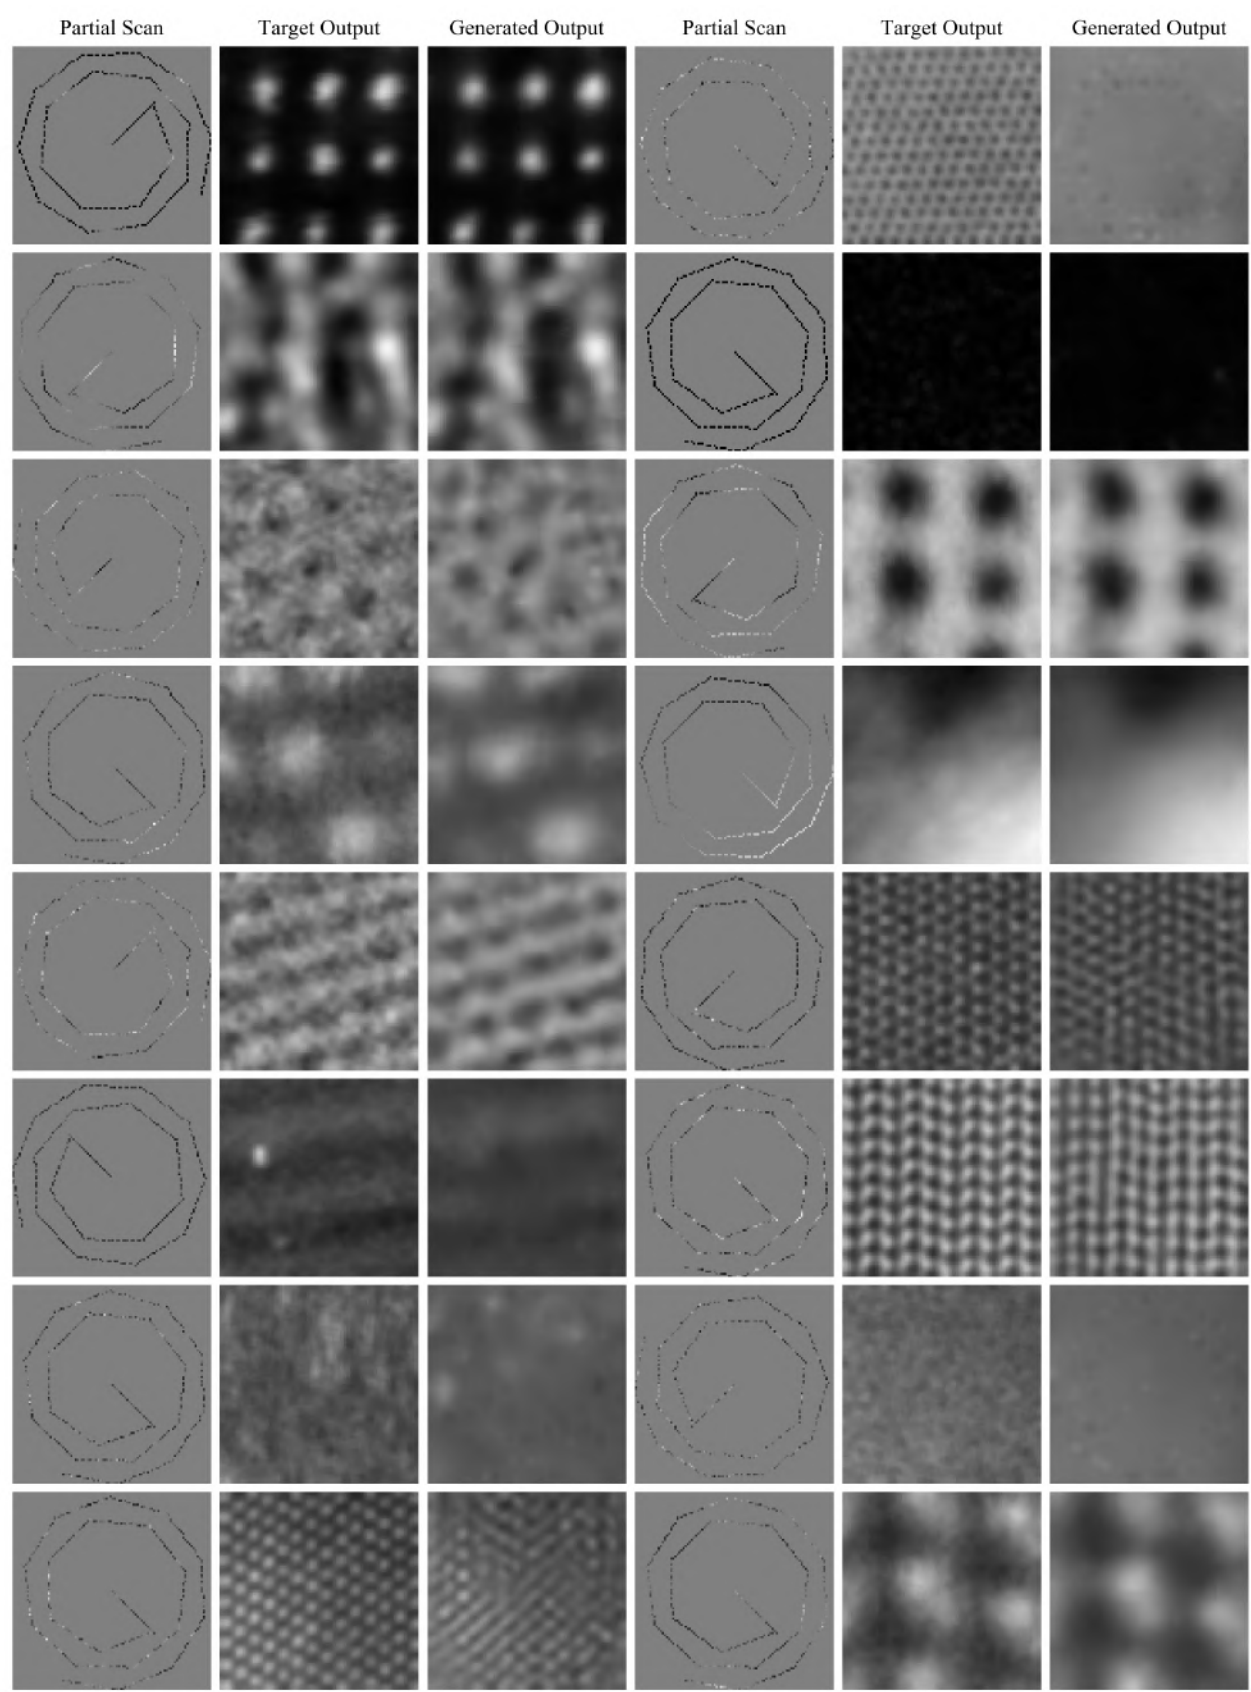

**Figure S6.** Test set 1/23.04 px coverage spiral partial scans, target outputs, and generated partial scan completions for  $96 \times 96$  crops from STEM images.

## References

1. Zaremba, W., Sutskever, I. & Vinyals, O. Recurrent Neural Network Regularization. *arXiv preprint arXiv:1409.2329* (2014).
2. Graves, A. *et al.* Hybrid Computing Using a Neural Network with Dynamic External Memory. *Nature* **538**, 471–476 (2016).
3. Jozefowicz, R., Zaremba, W. & Sutskever, I. An Empirical Exploration of Recurrent Network Architectures. In *International Conference on Machine Learning*, 2342–2350 (2015).
4. Pitis, S. Non-Zero Initial States for Recurrent Neural Networks. Online: <https://r2rt.com/non-zero-initial-states-for-recurrent-neural-networks.html> (2016).
5. DeepMind. Differentiable Neural Computer. Online: <https://github.com/deepmind/dnc> (2018).
6. Dumoulin, V. & Visin, F. A Guide to Convolution Arithmetic for Deep Learning. *arXiv preprint arXiv:1603.07285* (2016).
7. He, K., Zhang, X., Ren, S. & Sun, J. Deep Residual Learning for Image Recognition. CoRR abs/1512.03385 (2015).
8. Nair, V. & Hinton, G. E. Rectified Linear Units Improve Restricted Boltzmann Machines. In *Proceedings of the 27th International Conference on Machine Learning (ICML-10)*, 807–814 (2010).
9. Ioffe, S. & Szegedy, C. Batch Normalization: Accelerating Deep Network Training by Reducing Internal Covariate Shift. *arXiv preprint arXiv:1502.03167* (2015).
10. Glorot, X. & Bengio, Y. Understanding the Difficulty of Training Deep Feedforward Neural Networks. In *Proceedings of the Thirteenth International Conference on Artificial Intelligence and Statistics*, 249–256 (2010).
11. Kukačka, J., Golkov, V. & Cremers, D. Regularization for Deep Learning: A Taxonomy. *arXiv preprint arXiv:1710.10686* (2017).
12. Zhang, J., He, T., Sra, S. & Jadbabaie, A. Why Gradient Clipping Accelerates Training: A Theoretical Justification for Adaptivity. *arXiv preprint arXiv:1905.11881* (2019).
13. Gorbunov, E., Danilova, M. & Gasnikov, A. Stochastic Optimization with Heavy-Tailed Noise via Accelerated Gradient Clipping. *arXiv preprint arXiv:2005.10785* (2020).
14. Chen, X., Wu, Z. S. & Hong, M. Understanding Gradient Clipping in Private SGD: A Geometric Perspective. *arXiv preprint arXiv:2006.15429* (2020).
15. Menon, A. K., Rawat, A. S., Reddi, S. J. & Kumar, S. Can Gradient Clipping Mitigate Label Noise? In *International Conference on Learning Representations* (2019).
16. Smith, L. N. Cyclical Learning Rates for Training Neural Networks. In *2017 IEEE Winter Conference on Applications of Computer Vision (WACV)*, 464–472 (IEEE, 2017).
17. Ede, J. M. Warwick Electron Microscopy Datasets. *Mach. Learn. Sci. Technol.* **1**, 045003 (2020).
18. Vairalkar, M. K. & Nimbhorkar, S. Edge Detection of Images Using Sobel Operator. *Int. J. Emerg. Technol. Adv. Eng.* **2**, 291–293 (2012).
19. Zhao, H., Gallo, O., Frosio, I. & Kautz, J. Loss Functions for Neural Networks for Image Processing. *arXiv preprint arXiv:1511.08861* (2015).
20. Gui, J., Sun, Z., Wen, Y., Tao, D. & Ye, J. A Review on Generative Adversarial Networks: Algorithms, Theory, and Applications. *arXiv preprint arXiv:2001.06937* (2020).
21. Saxena, D. & Cao, J. Generative Adversarial Networks (GANs): Challenges, Solutions, and Future Directions. *arXiv preprint arXiv:2005.00065* (2020).
22. Pan, Z. *et al.* Recent Progress on Generative Adversarial Networks (GANs): A Survey. *IEEE Access* **7**, 36322–36333 (2019).
23. Wang, Z., She, Q. & Ward, T. E. Generative Adversarial Networks: A Survey and Taxonomy. *arXiv preprint arXiv:1906.01529* (2019).
24. Ede, J. M. & Beanland, R. Partial Scanning Transmission Electron Microscopy with Deep Learning. *arXiv preprint arXiv:1910.10467* (2020).
25. Grund Pihlgren, G., Sandin, F. & Liwicki, M. Improving Image Autoencoder Embeddings with Perceptual Loss. In *International Joint Conference on Neural Networks* (2020).

26. Ede, J. M. & Beanland, R. Adaptive Learning Rate Clipping Stabilizes Learning. *Mach. Learn. Sci. Technol.* **1**, 015011 (2020).
27. Jia, Y., Wu, Z., Xu, Y., Ke, D. & Su, K. Long Short-Term Memory Projection Recurrent Neural Network Architectures for Piano's Continuous Note Recognition. *J. Robotics* **2017** (2017).
28. Ruder, S. An Overview of Gradient Descent Optimization Algorithms. *arXiv preprint arXiv:1609.04747* (2016).
29. Heess, N., Hunt, J. J., Lillicrap, T. P. & Silver, D. Memory-Based Control with Recurrent Neural Networks. *arXiv preprint arXiv:1512.04455* (2015).
30. Li, M., Soltanolkotabi, M. & Oymak, S. Gradient Descent with Early Stopping is Provably Robust to Label Noise for Overparameterized Neural Networks. In *International Conference on Artificial Intelligence and Statistics*, 4313–4324 (2020).
31. Flynn, T., Yu, K. M., Malik, A., D'Imperio, N. & Yoo, S. Bounding the Expected Run-Time of Nonconvex Optimization with Early Stopping. *arXiv preprint arXiv:2002.08856* (2020).
32. Sang, X. *et al.* Dynamic Scan Control in STEM: Spiral Scans. *Adv. Struct. Chem. Imaging* **2**, 6 (2017).
33. Zhang, C., Berkels, B., Wirth, B. & Voyles, P. M. Joint Denoising and Distortion Correction for Atomic Column Detection in Scanning Transmission Electron Microscopy Images. *Microsc. Microanal.* **23**, 164–165 (2017).
34. Jin, P. & Li, X. Correction of Image Drift and Distortion in a Scanning Electron Microscopy. *J. Microsc.* **260**, 268–280 (2015).
35. Zhu, J.-Y., Park, T., Isola, P. & Efros, A. A. Unpaired Image-to-Image Translation Using Cycle-Consistent Adversarial Networks. In *Proceedings of the IEEE International Conference on Computer Vision*, 2223–2232 (2017).
