# Supplementary material for: Advances in Electron Microscopy with Deep Learning
Source: arXiv:2101.01178 source file (2021-03-11)
Supplement: Supplementary file 3 [file paper_wemd_supplementary.pdf]

# Supplementary Information: Warwick Electron Microscopy Datasets

Jeffrey M. Ede<sup>1,\*</sup>

<sup>1</sup>University of Warwick, Department of Physics, Coventry, CV4 7AL, UK

\*j.m.ede@warwick.ac.uk

## S1 Additional Visualizations

Figure numbers for a variety of two-dimensional tSNE visualisations are tabulated in table S1 to ease comparison. Visualizations are for the first 50 principal components extracted by a scikit-learn<sup>1</sup> implementation of probabilistic PCA, means encoded in 64-dimensional VAE latent spaces without modified tSNE losses to account for standard deviations, and means encoded in 64-dimensional VAE latent spaces with modified tSNE losses to account for standard deviations. Interactive versions of tSNE visualizations that display data when map points are hovered over are also available for every visualization<sup>2</sup>. In addition, our source code, graph points and datasets are openly available.

| Dataset                        | PCA | VAE $\{\mu\}$ | VAE $\{\mu, \sigma\}$ |
|--------------------------------|-----|---------------|-----------------------|
| STEM 96×96                     | S1  | S7            | 3 (main article)      |
| STEM 96×96 Crops               | S2  | S8            | S10                   |
| TEM 96×96                      | S3  | S9            | 4 (main article)      |
| Wavefunctions 96×96            | S4  | -             | -                     |
| Wavefunctions 96×96 Restricted | S5  | -             | -                     |
| Wavefunctions 96×96 Single     | S6  | -             | -                     |

**Table S1.** To ease comparison, we have tabulated figure numbers for tSNE visualizations. Visualizations are for principal components, VAE latent space means, and VAE latent space means weighted by standard deviations..

Visualization of complex exit wavefunctions is complicated by the display of their real and imaginary components. However, real and imaginary components are related<sup>3</sup>, and can be visualized in the same image by displaying them in different colour channels. For example, we show real and imaginary components in red and blue colour channels, respectively, in figures S4-S6. Note that a couple of extreme points are cropped from some of the tSNE visualizations of principal components in figures S1-S6. However, this only affected ~0.01% of points and therefore does not have a substantial effect on visualizations. In contrast, tSNE visualizations of VAE latent spaces did not have extreme points.

## S2 Uniformly Separated tSNE

Limitedly, most tSNE visualizations do not fully utilize whitespace. This is problematic as space is often limited in journals, websites and other media. As a result, we propose algorithm 1 to uniformly separate map points. This increases whitespace utilization while keeping clustered points together. Example applications are shown in figures S11-S13, where images nearest points on a regular grid are shown at grid points. Uniformly separating map points removes information about pairwise distances encoded in the tSNE distributions. However, distances and cluster sizes in tSNE visualizations are not overly meaningful<sup>4</sup>. Overall, we think that uniformly separated tSNE is an interesting option that could be improved by further development. To this end, our source code and graph points for uniformly separated tSNE visualizations are openly available<sup>2</sup>.

## S3 Image Search Engines

Our VAEs can be used as the basis of image search engines. To find similar images, we compute Euclidean distances between means encoded for search inputs and images in the STEM or TEM datasets, then select images at lowest distances. Examples of top-5 search results for various input images are shown in figure S14 and figure S15 for TEM and STEM, respectively. Search results are most accurate for common images and are less accurate for unusual images. The main difference between the performance of our search engines and Google, Bing or other commercial image search engines is the result of commercial ANNs being trained with over 100× more training data, 3500× more computational resources and larger images c.f. Xception<sup>5</sup>.

However, the performance of our search engines is okay and our VAEs could easily be scaled up. Our source code, pretrained models and VAE encodings for each dataset are openly available<sup>2</sup>.

---

**Algorithm 1** Two-dimensional Bayesian inverse transformed tSNE. We default to a  $h = w = 25$  grid.

---

Initialize  $N$  two-dimensional tSNE map points,  $\mathbf{X} = \{\mathbf{x}_1, \dots, \mathbf{x}_N\}$ , where  $\mathbf{x}_i = \{x_{i1}, x_{i2}\}$ .

Linearly transform dimensions to have values in  $[0, 1]$ ,

$$x_{ij} \leftarrow \frac{x_{ij} - \min_i(x_{ij})}{\max_i(x_{ij}) - \min_i(x_{ij})}. \quad (1)$$

Divide points into an evenly spaced grid with  $h \times w$  cells.

Compute number of points in each cell,  $n_{ab}$ ,  $a \in [1, h]$ ,  $b \in [1, w]$ .

Cumulative numbers of points using the recurrent relations,

$$c_a = c_{a-1} + \sum_{b=1}^w n_{ab}, \quad (2)$$

$$c_{b|a} = c_{b-1|a} + n_{ab}, \quad (3)$$

where  $c_0 = c_{0|a} = 0$ .

Estimate Bayesian conditional cumulative distribution functions,

$$C_a = c_a / c_h, \quad (4)$$

$$C_{b|a} = c_{b|a} / c_a. \quad (5)$$

Map grid points,  $\{(a - 0.5)/h, (b - 0.5)/w\}$ , to distribution points,  $\{(u - 0.5)/h, (v - 0.5)/w\}$ , where  $u$  and  $v$  are minimum values that satisfy

$$(a - 0.5)/h \leq C_u, \quad (6)$$

$$(b - 0.5)/w \leq C_{v|u}. \quad (7)$$

Interpolate uniformly separated grid positions,  $\mathbf{Y}$ , for  $\mathbf{X}$  based on pairs of grid and distribution points. We use Clough-Tocher cubic Bezier interpolation<sup>6</sup>.

---

## References

1. Pedregosa, F. *et al.* Scikit-learn: Machine Learning in Python. *J. Mach. Learn. Res.* **12**, 2825–2830 (2011).
2. Ede, J. M. Visualization of Electron Microscopy Datasets with Deep Learning. Online: <https://github.com/Jeffrey-Ede/datasets>, DOI: [10.5281/zenodo.3834197](https://doi.org/10.5281/zenodo.3834197) (2020).
3. Ede, J. M., Peters, J. J. P., Sloan, J. & Beanland, R. Exit Wavefunction Reconstruction from Single Transmission Electron Micrographs with Deep Learning. *arXiv preprint arXiv:2001.10938* (2020).
4. Wattenberg, M., Viégas, F. & Johnson, I. How to Use t-SNE Effectively. *Distill* **1**, e2 (2016).
5. Chollet, F. Xception: Deep Learning with Depthwise Separable Convolutions. In *Proceedings of the IEEE Conference on Computer Vision and Pattern Recognition*, 1251–1258 (2017).
6. Alfeld, P. A Trivariate Clough—Tocher Scheme for Tetrahedral Data. *Comput. Aided Geom. Des.* **1**, 169–181 (1984).

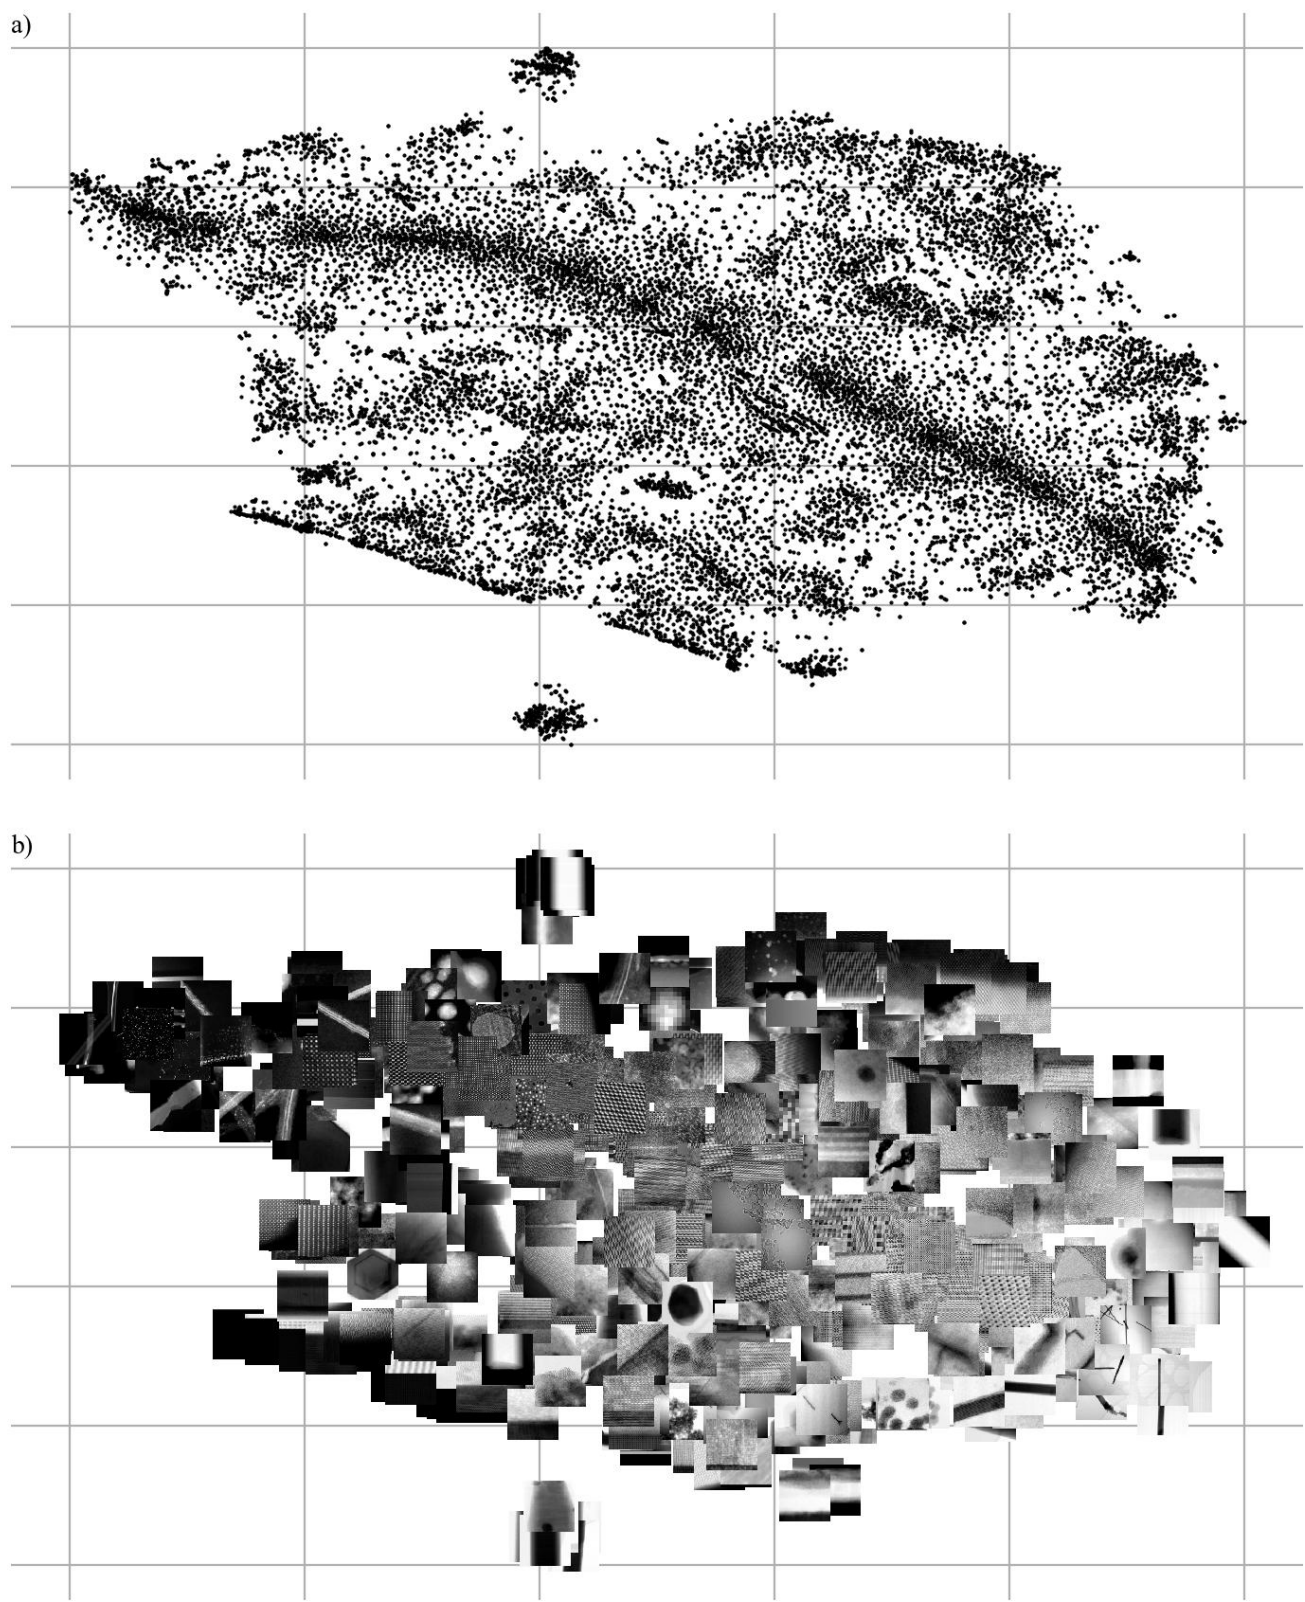

**Figure S1.** Two-dimensional tSNE visualization of the first 50 principal components of 19769 STEM images that have been downsampled to  $96 \times 96$ . The same grid is used to show a) map points and b) images at 500 randomly selected points.

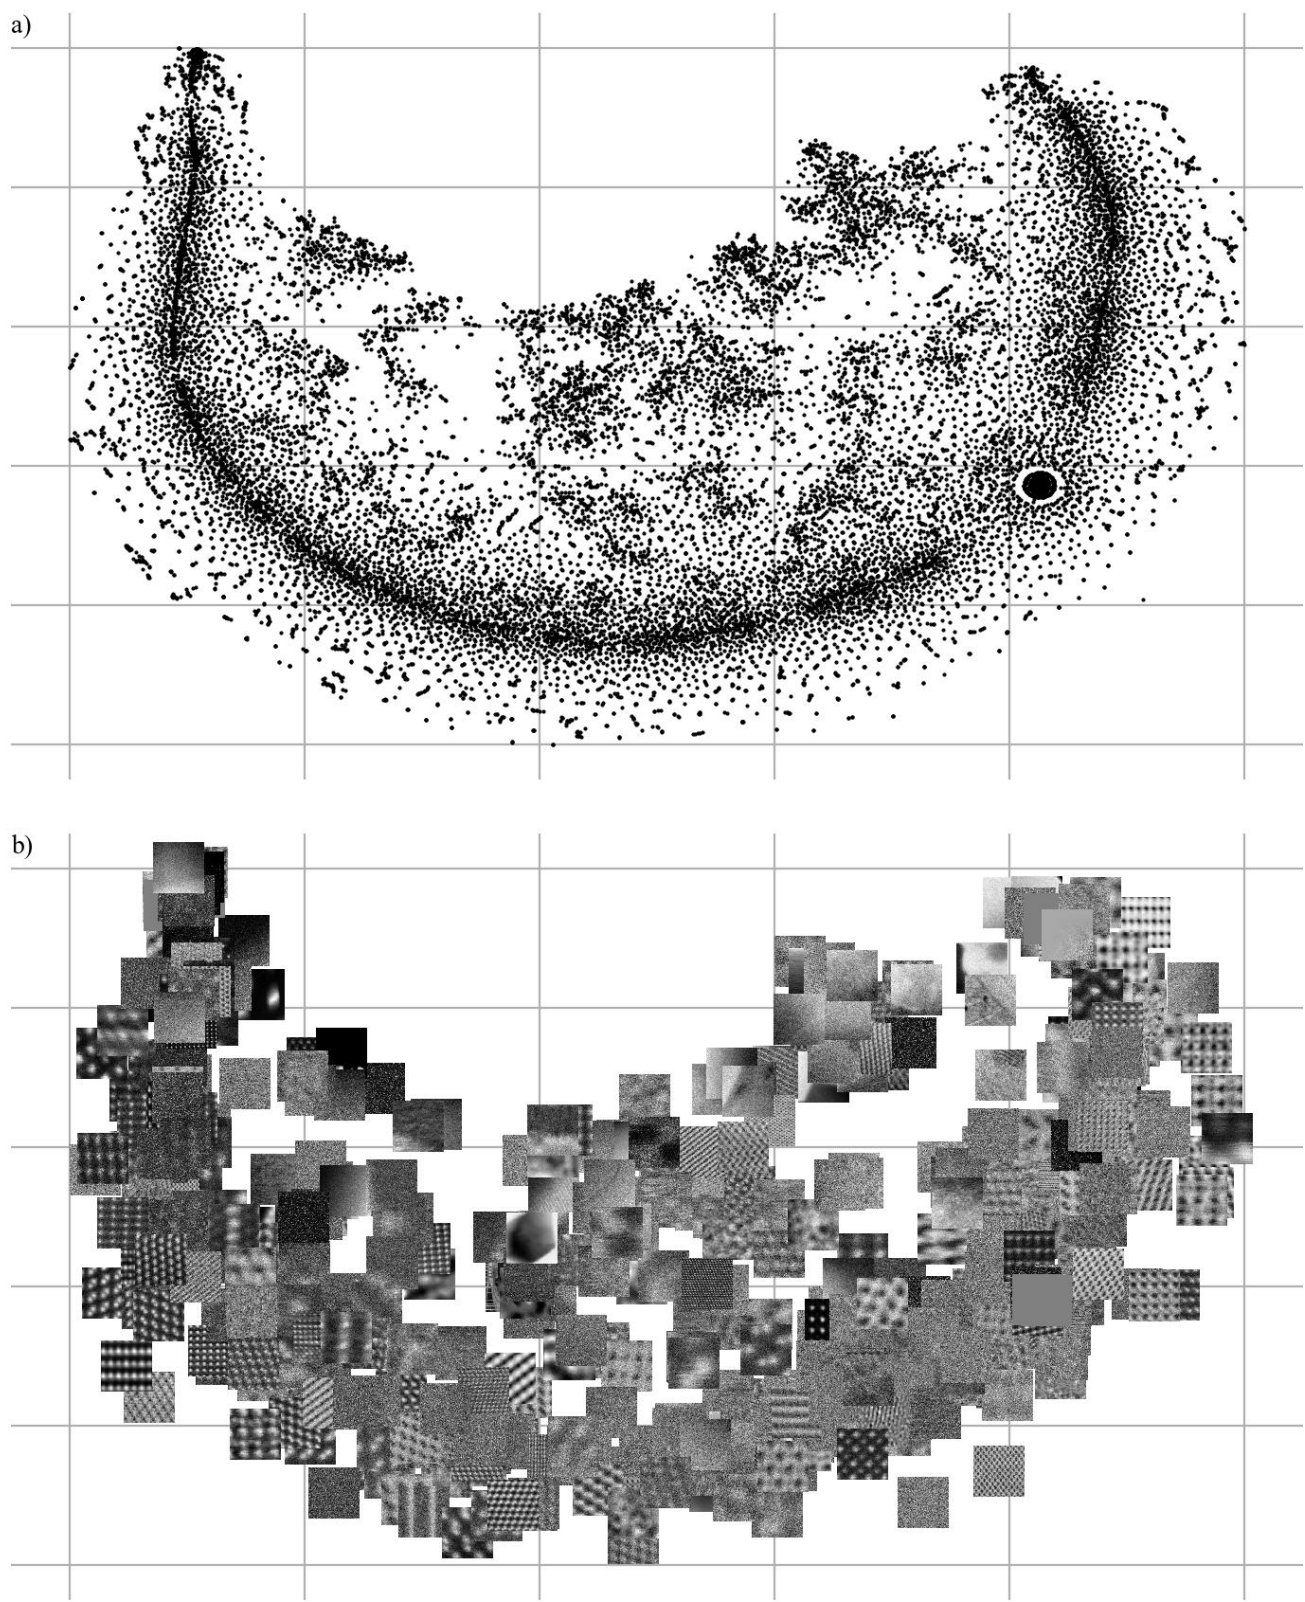

**Figure S2.** Two-dimensional tSNE visualization of the first 50 principal components of 19769  $96 \times 96$  crops from STEM images. The same grid is used to show a) map points and b) images at 500 randomly selected points.

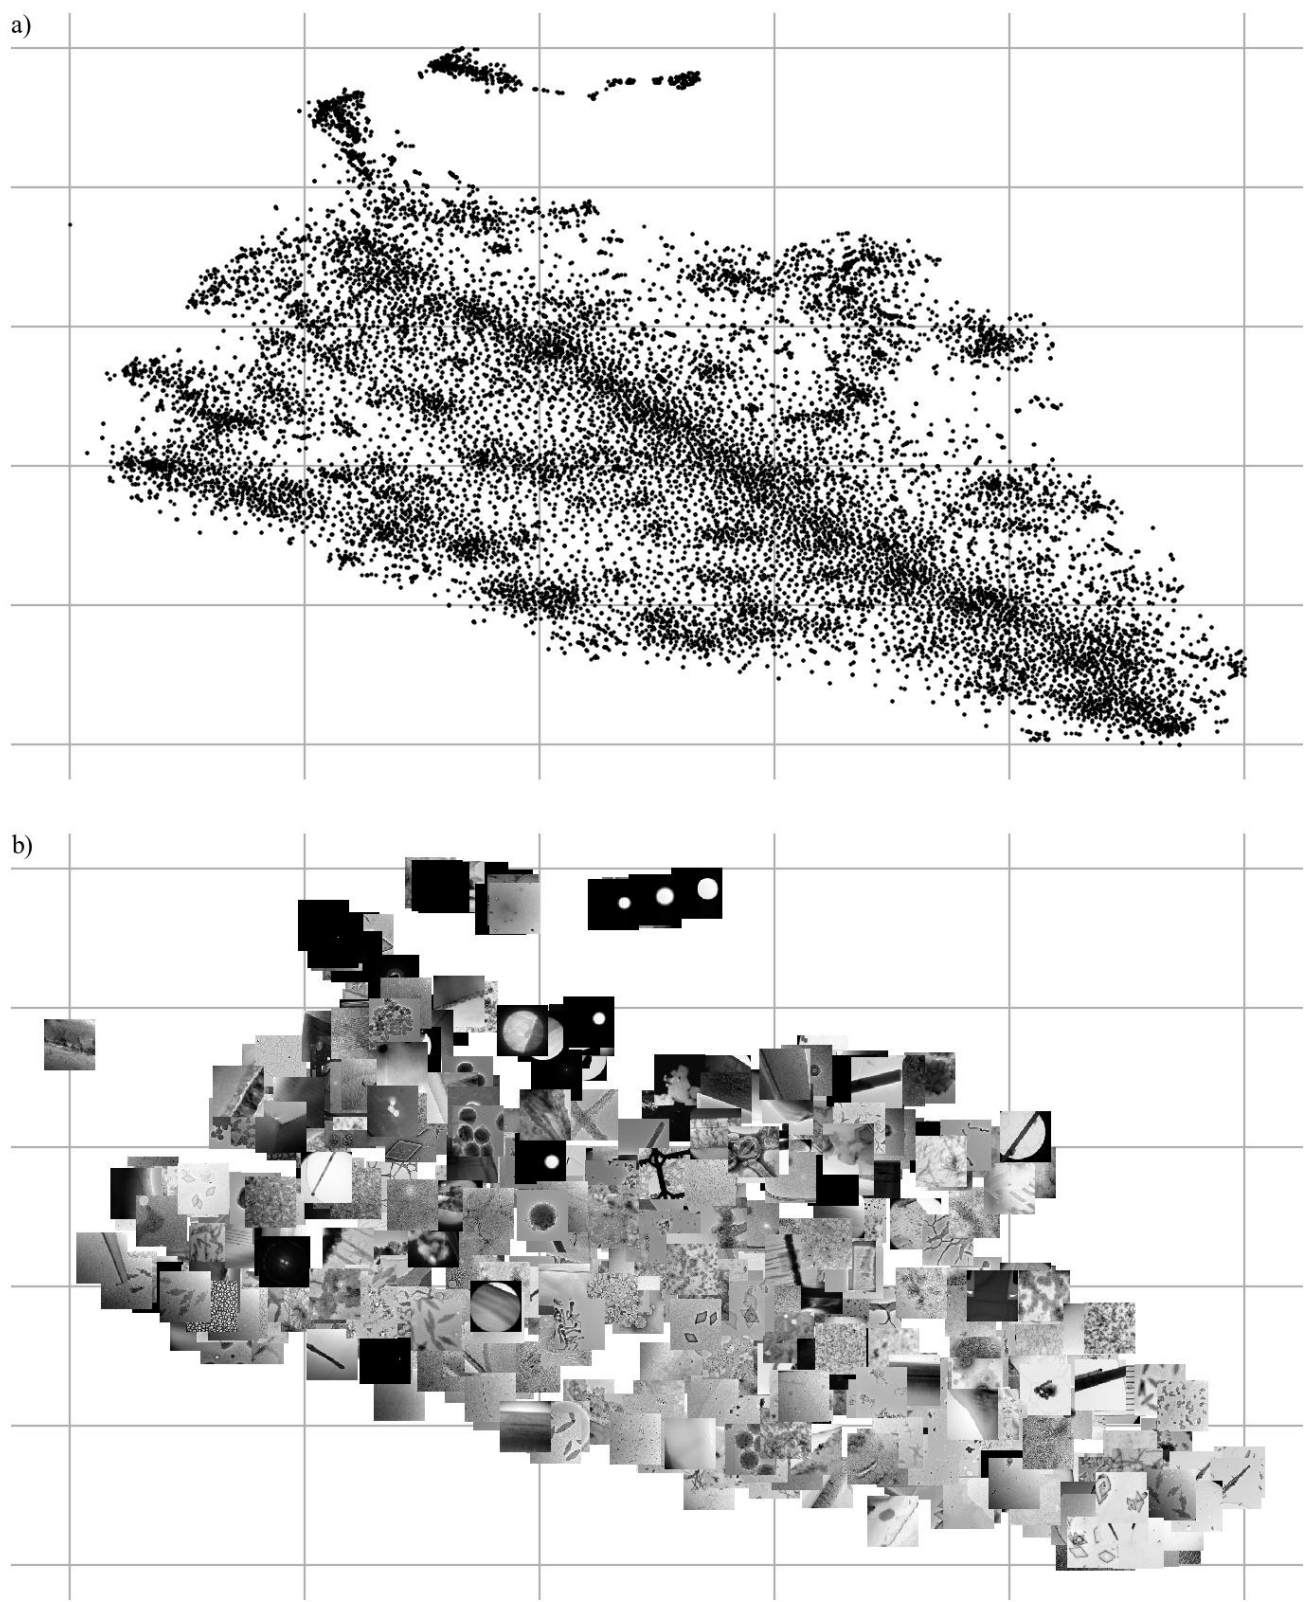

**Figure S3.** Two-dimensional tSNE visualization of the first 50 principal components of 17266 TEM images that have been downsampled to  $96 \times 96$ . The same grid is used to show a) map points and b) images at 500 randomly selected points.

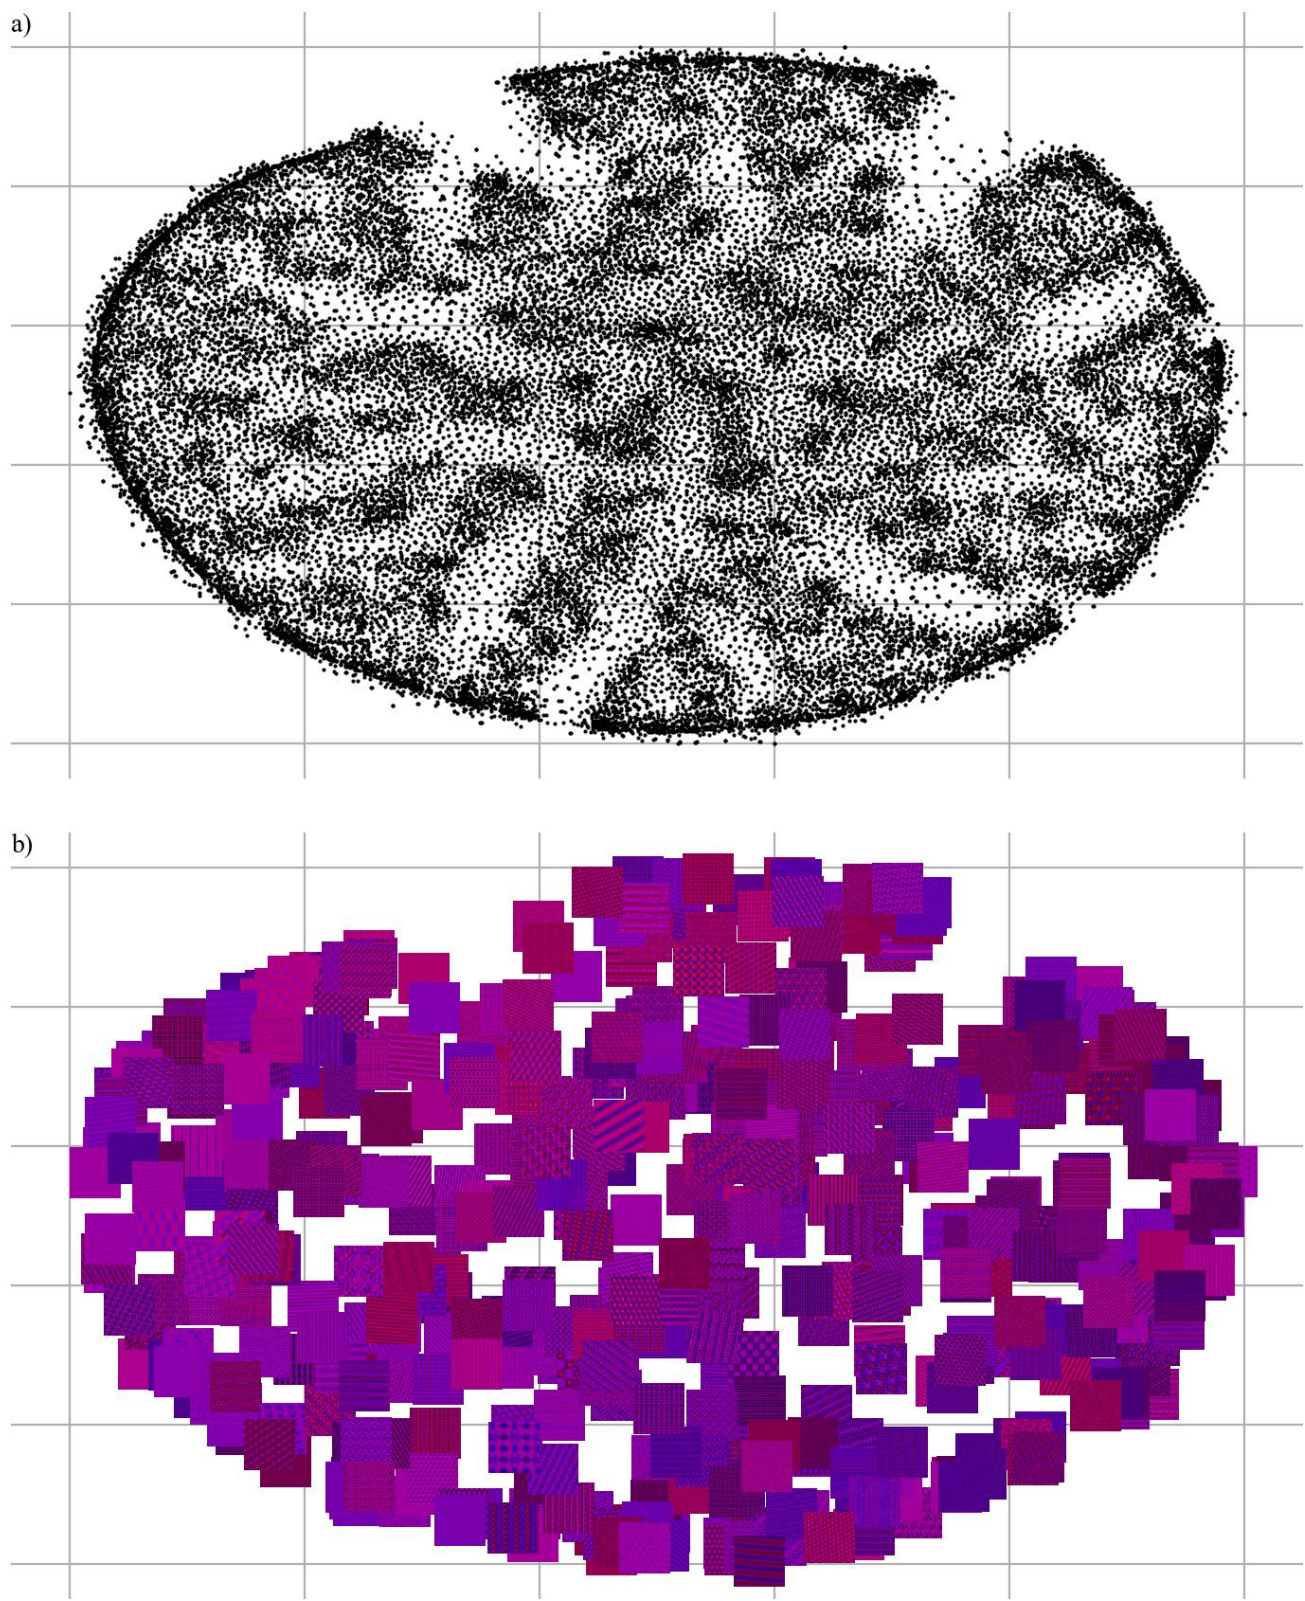

**Figure S4.** Two-dimensional tSNE visualization of the first 50 principal components of 36324 exit wavefunctions that have been downsampled to  $96 \times 96$ . Wavefunctions were simulated for thousands of materials and a large range of physical hyperparameters. The same grid is used to show a) map points and b) wavefunctions at 500 randomly selected points. Red and blue colour channels show real and imaginary components, respectively.

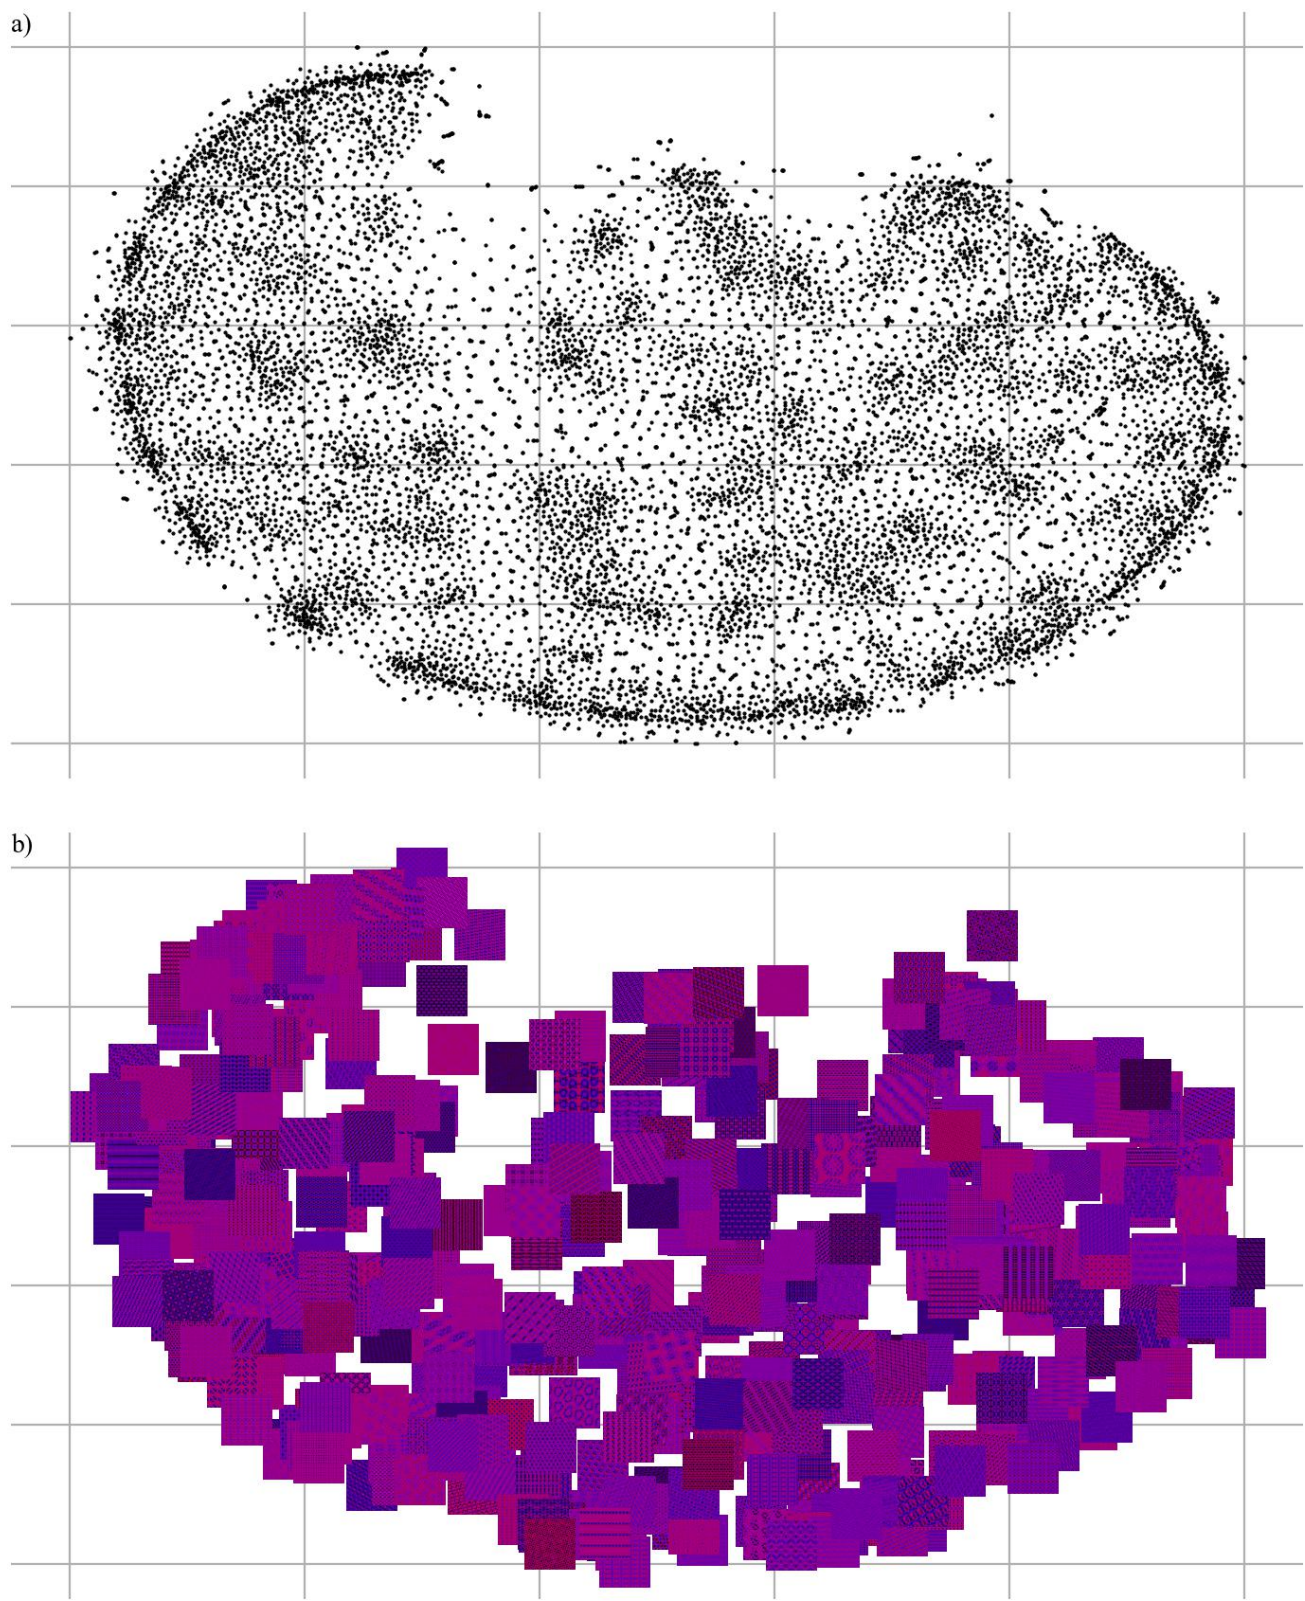

**Figure S5.** Two-dimensional tSNE visualization of the first 50 principal components of 11870 exit wavefunctions that have been downsampled to  $96 \times 96$ . Wavefunctions were simulated for thousands of materials and a small range of physical hyperparameters. The same grid is used to show a) map points and b) wavefunctions at 500 randomly selected points. Red and blue colour channels show real and imaginary components, respectively.

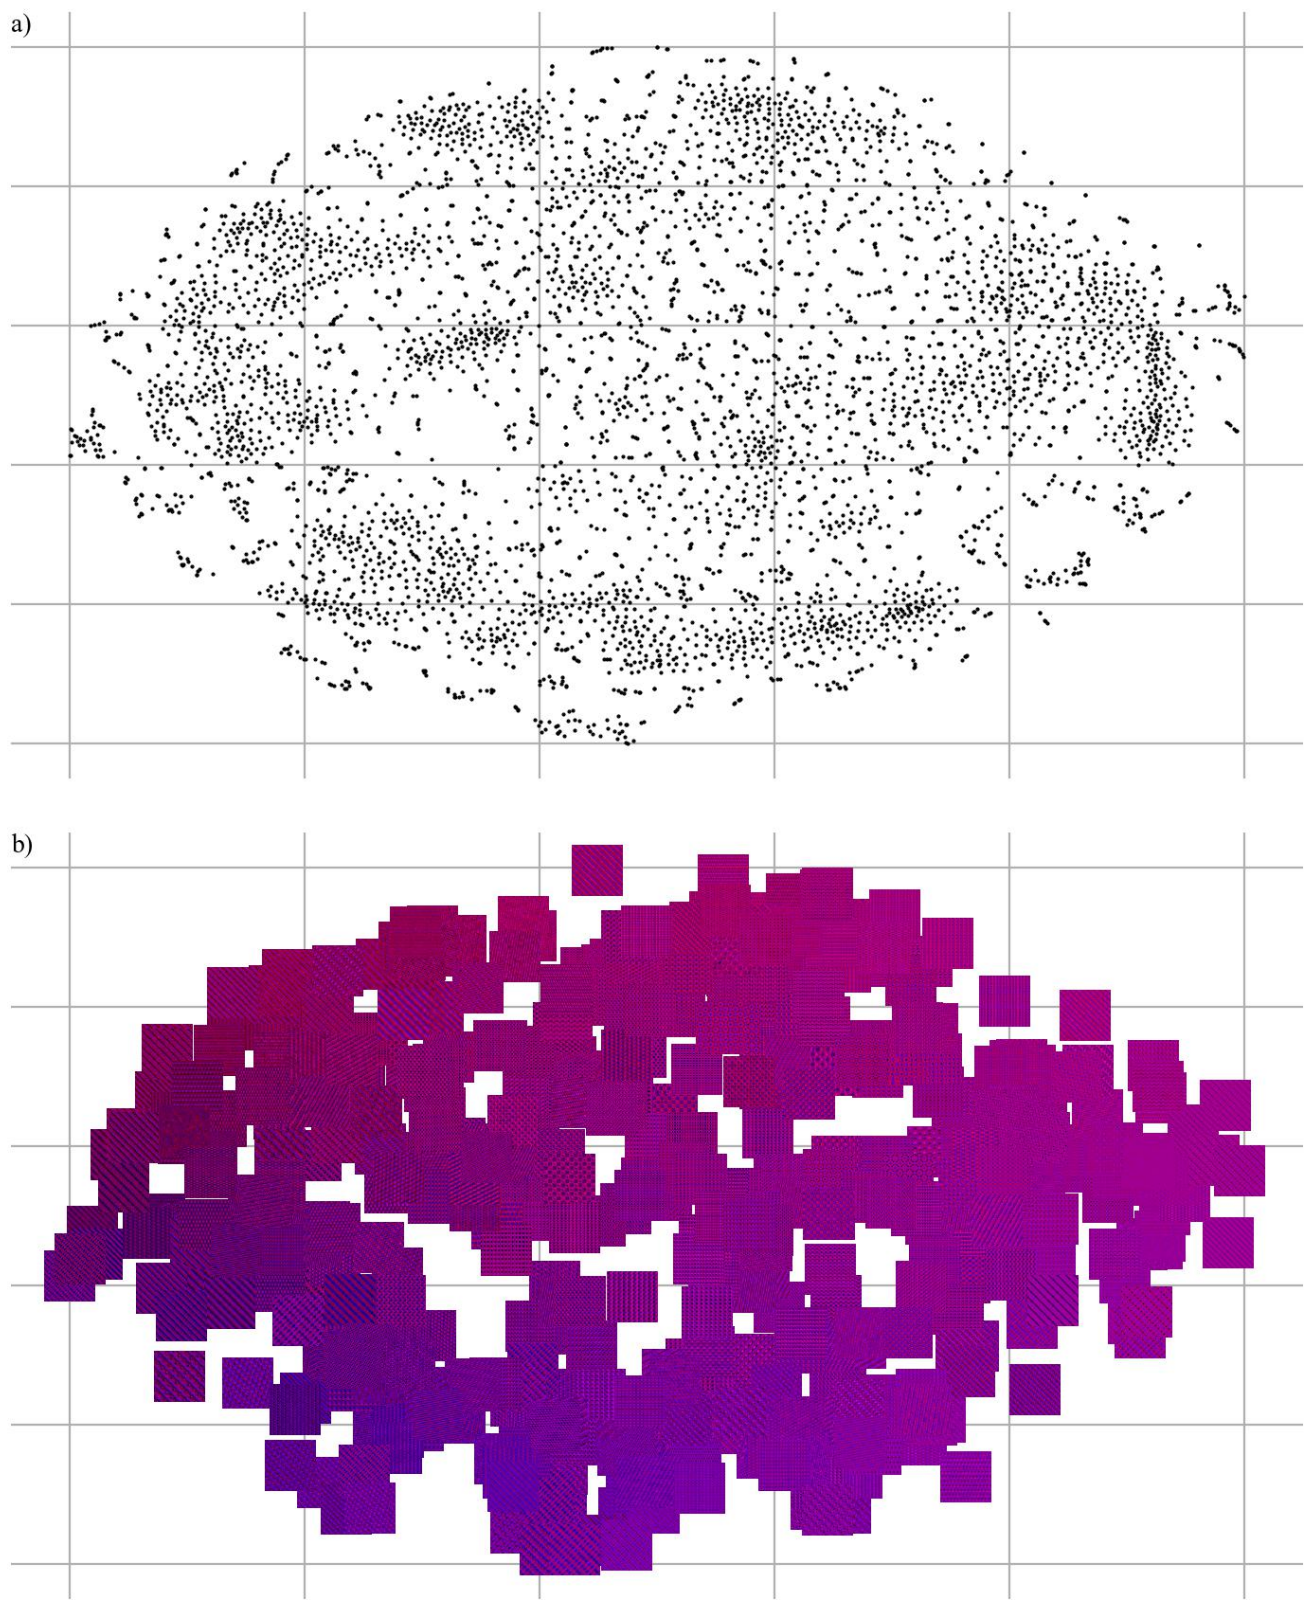

**Figure S6.** Two-dimensional tSNE visualization of the first 50 principal components of 4825 exit wavefunctions that have been downsampled to  $96 \times 96$ . Wavefunctions were simulated for thousands of materials and a small range of physical hyperparameters. The same grid is used to show a) map points and b) wavefunctions at 500 randomly selected points. Red and blue colour channels show real and imaginary components, respectively.

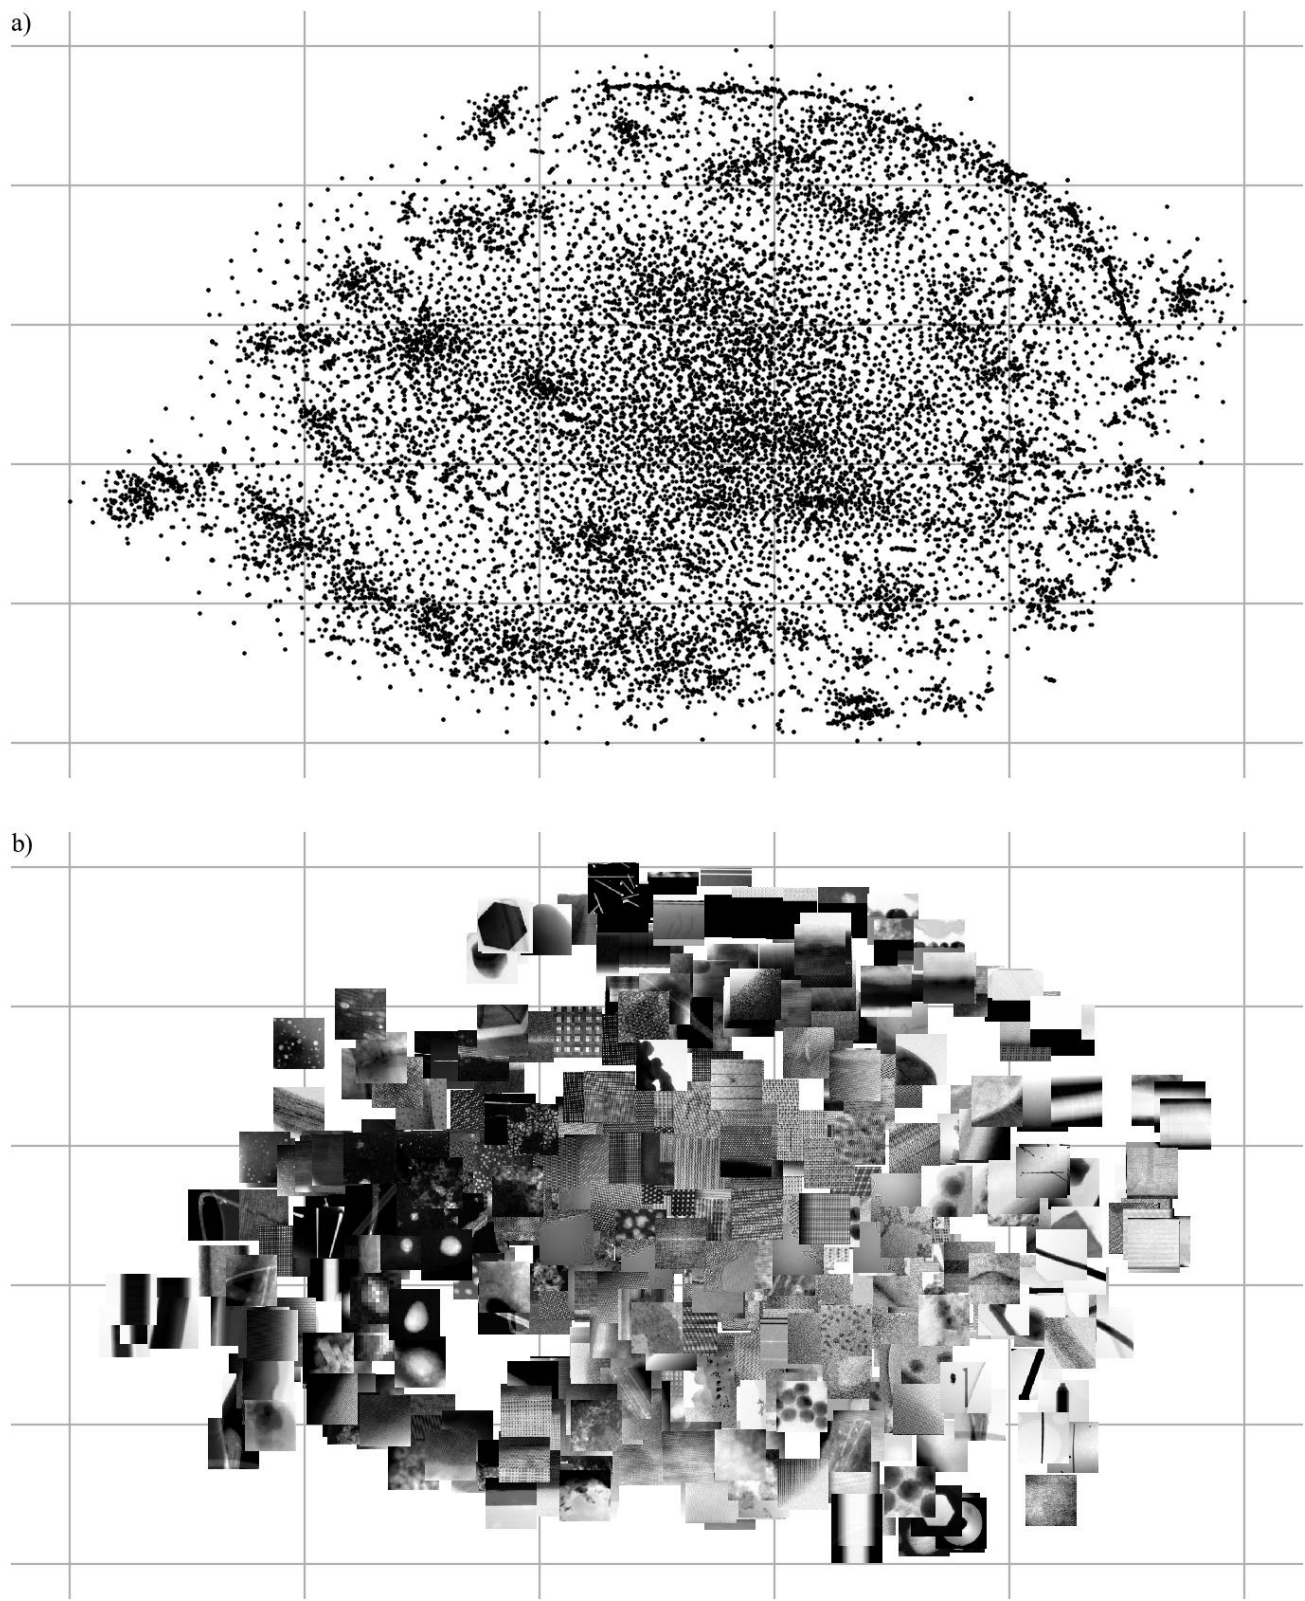

**Figure S7.** Two-dimensional tSNE visualization of means parameterized by 64-dimensional VAE latent spaces for 19769 STEM images that have been downsampled to  $96 \times 96$ . The same grid is used to show a) map points and b) images at 500 randomly selected points.

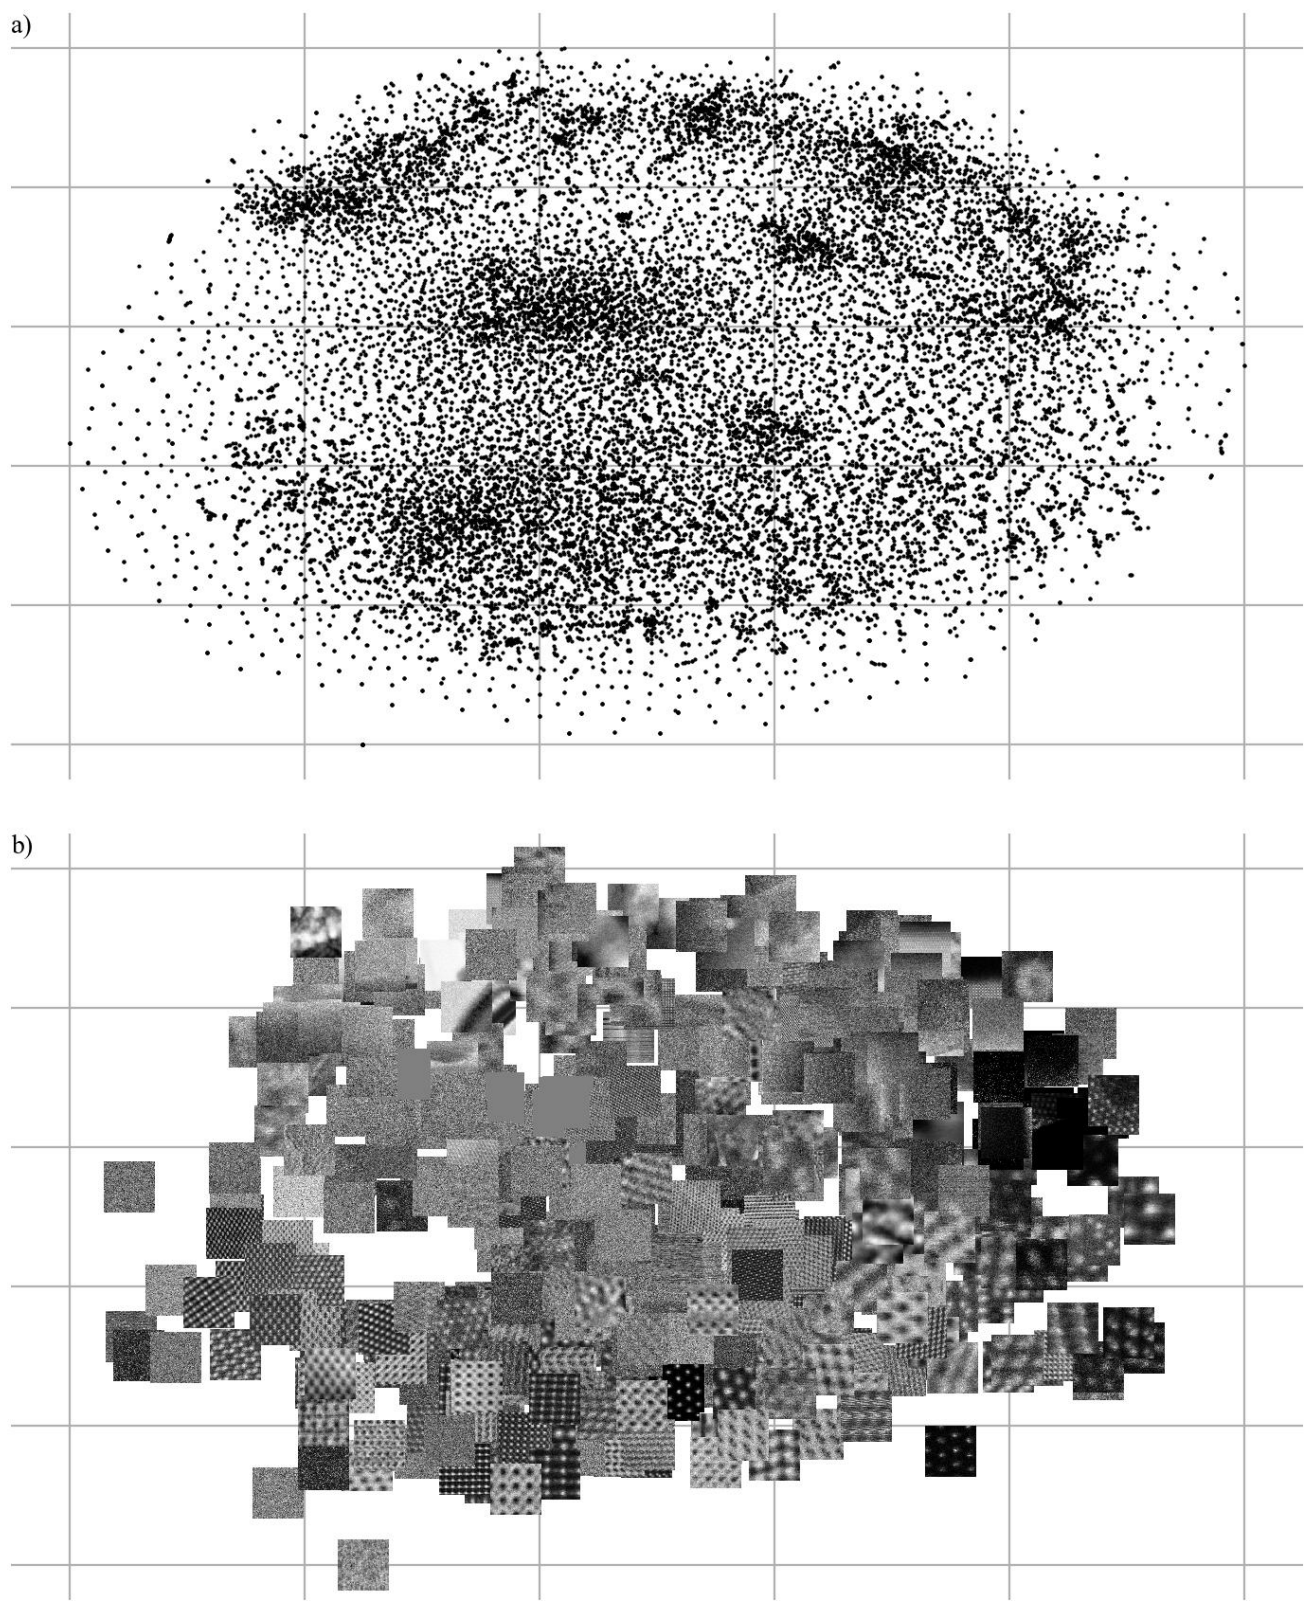

**Figure S8.** Two-dimensional tSNE visualization of means parameterized by 64-dimensional VAE latent spaces for 19769  $96 \times 96$  crops from STEM images. The same grid is used to show a) map points and b) images at 500 randomly selected points.

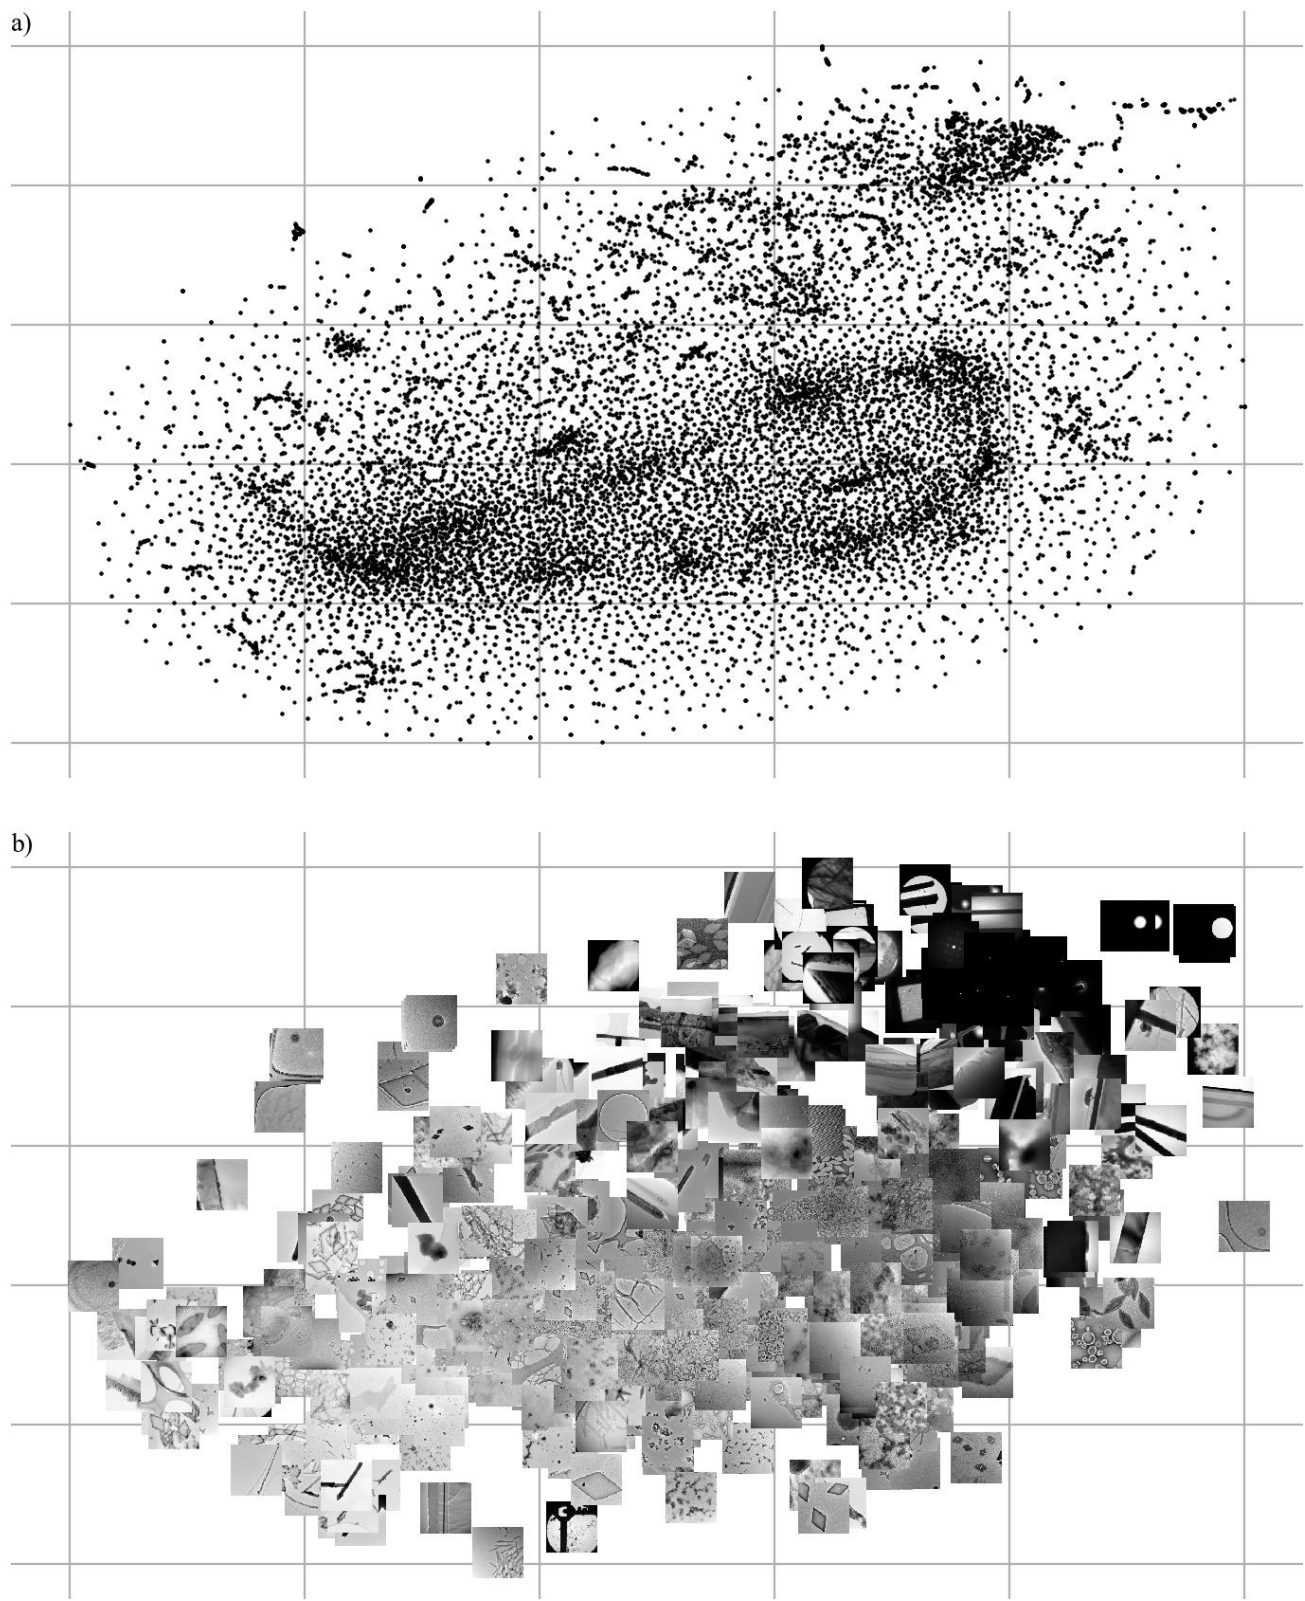

**Figure S9.** Two-dimensional tSNE visualization of means parameterized by 64-dimensional VAE latent spaces for 19769 TEM images that have been downsampled to  $96 \times 96$ . The same grid is used to show a) map points and b) images at 500 randomly selected points.

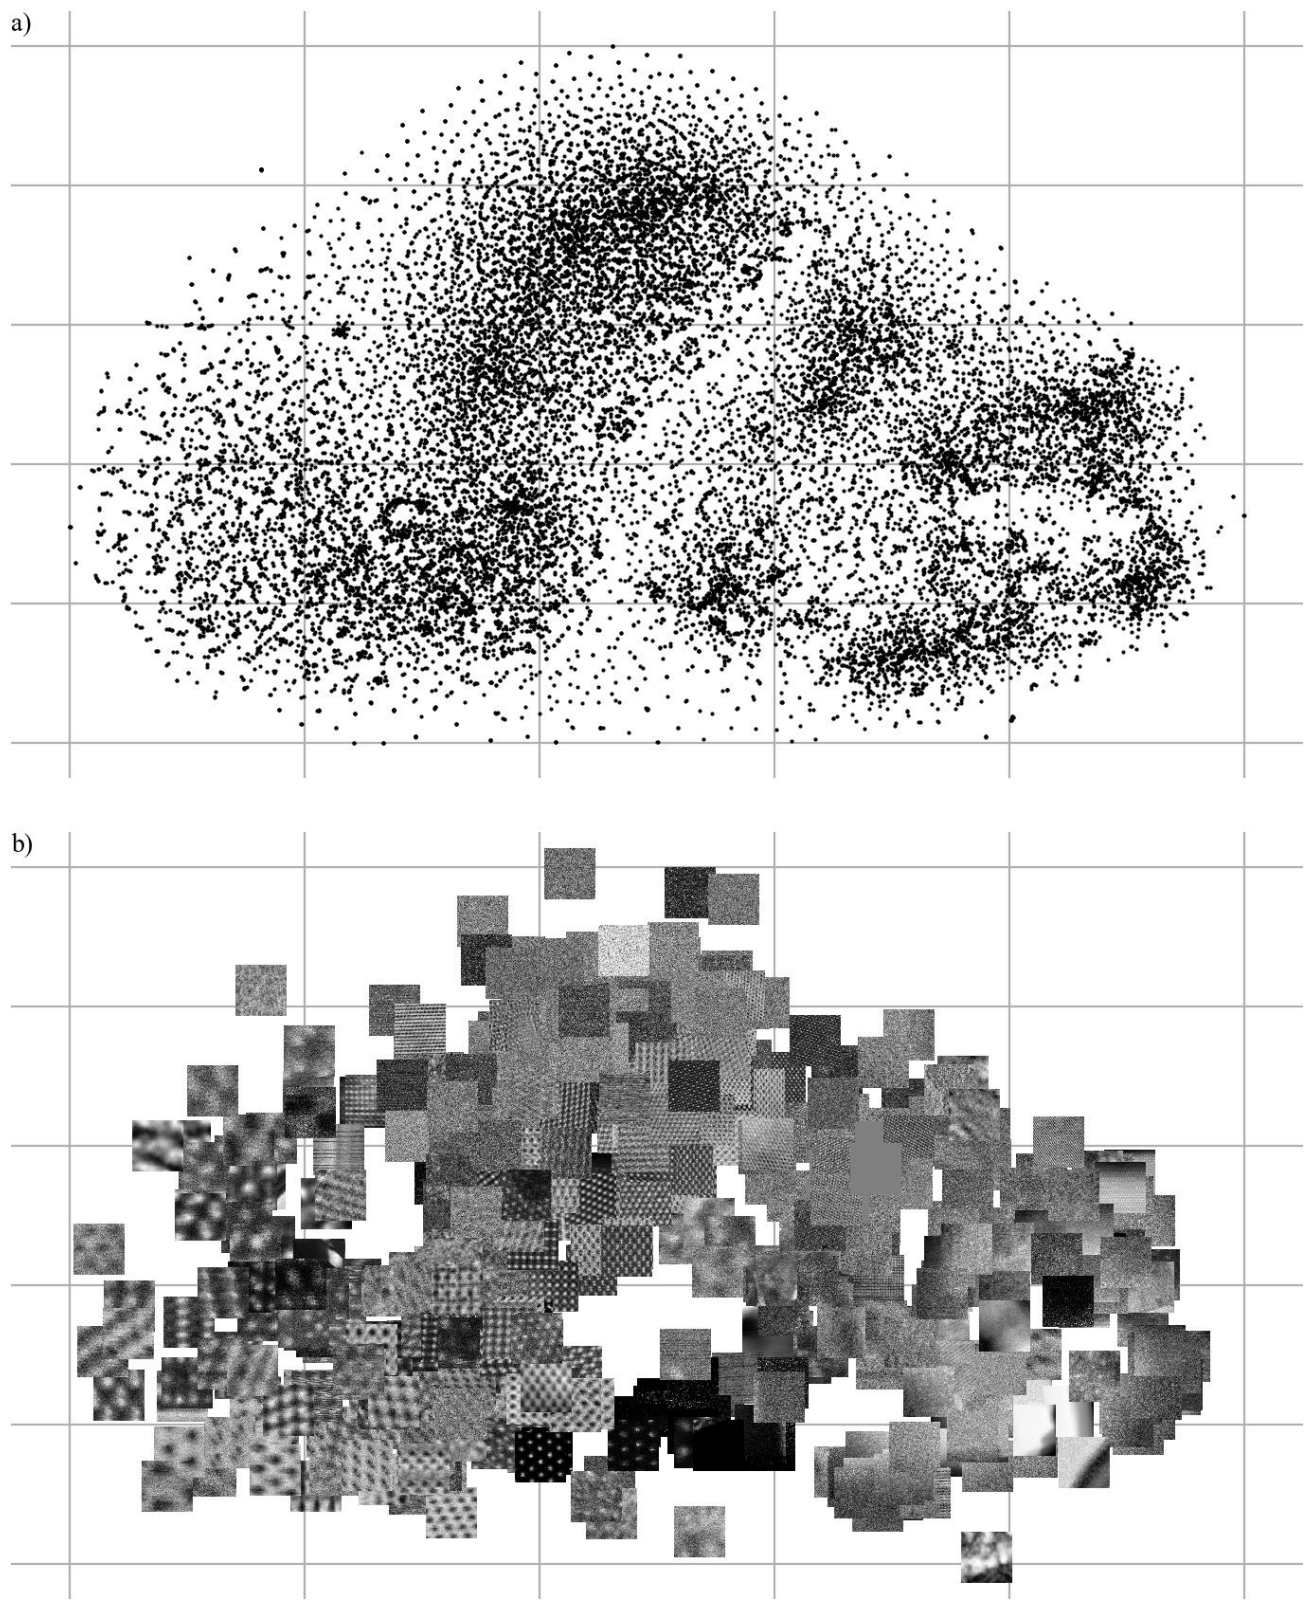

**Figure S10.** Two-dimensional tSNE visualization of means and standard deviations parameterized by 64-dimensional VAE latent spaces for 19769  $96 \times 96$  crops from STEM images. The same grid is used to show a) map points and b) images at 500 randomly selected points.

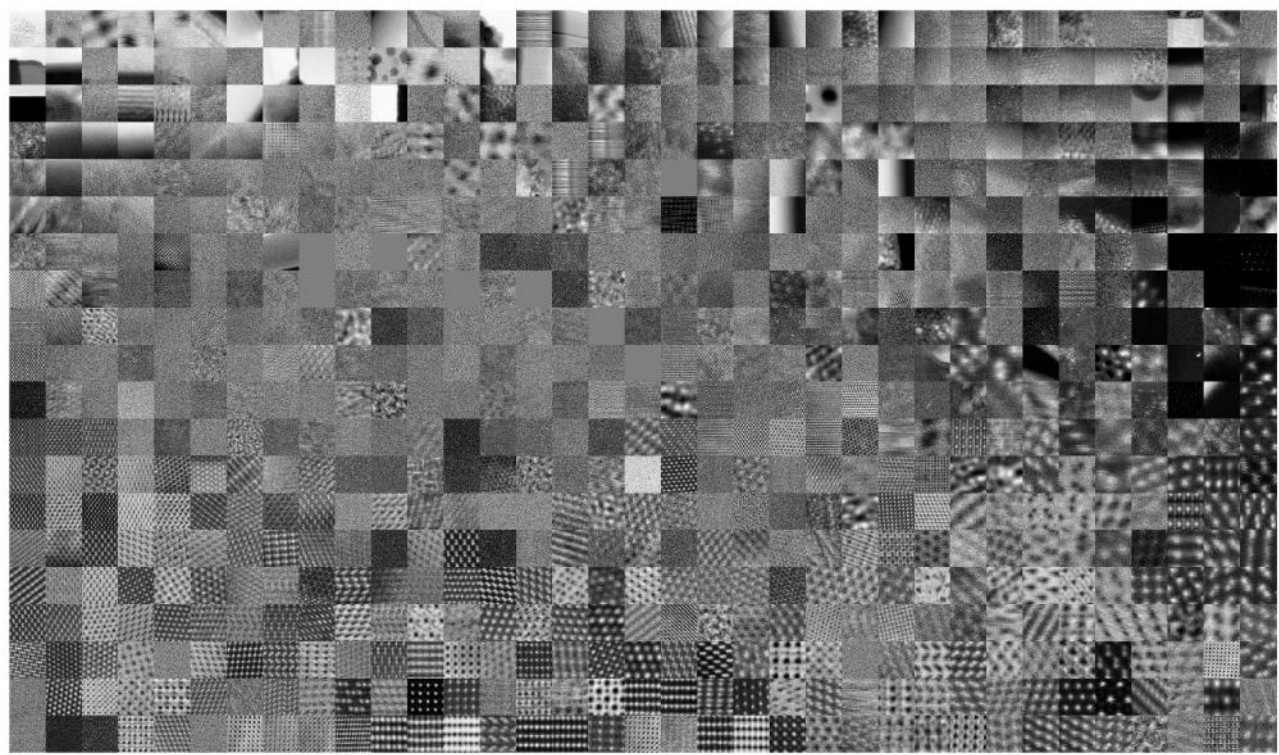

**Figure S11.** Two-dimensional uniformly separated tSNE visualization of 64-dimensional VAE latent spaces for 19769  $96 \times 96$  crops from STEM images.

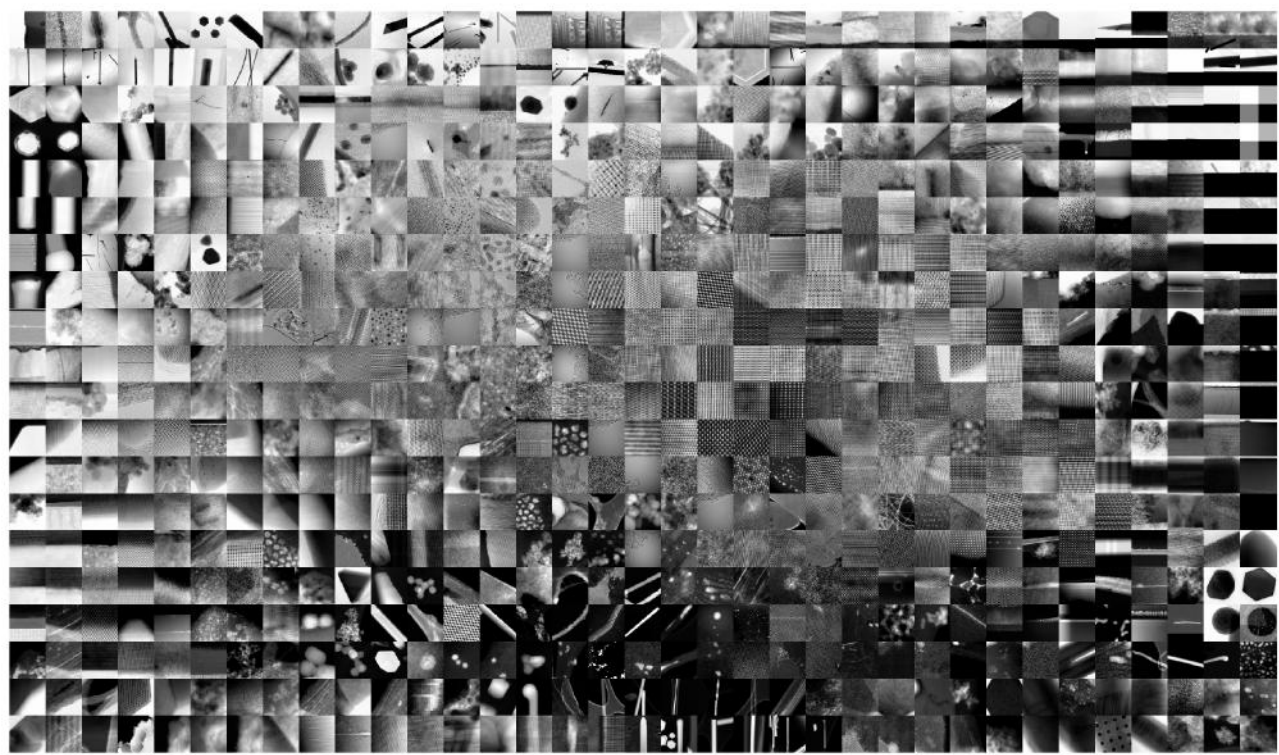

**Figure S12.** Two-dimensional uniformly separated tSNE visualization of 64-dimensional VAE latent spaces for 19769 STEM images that have been downsampled to  $96 \times 96$ .

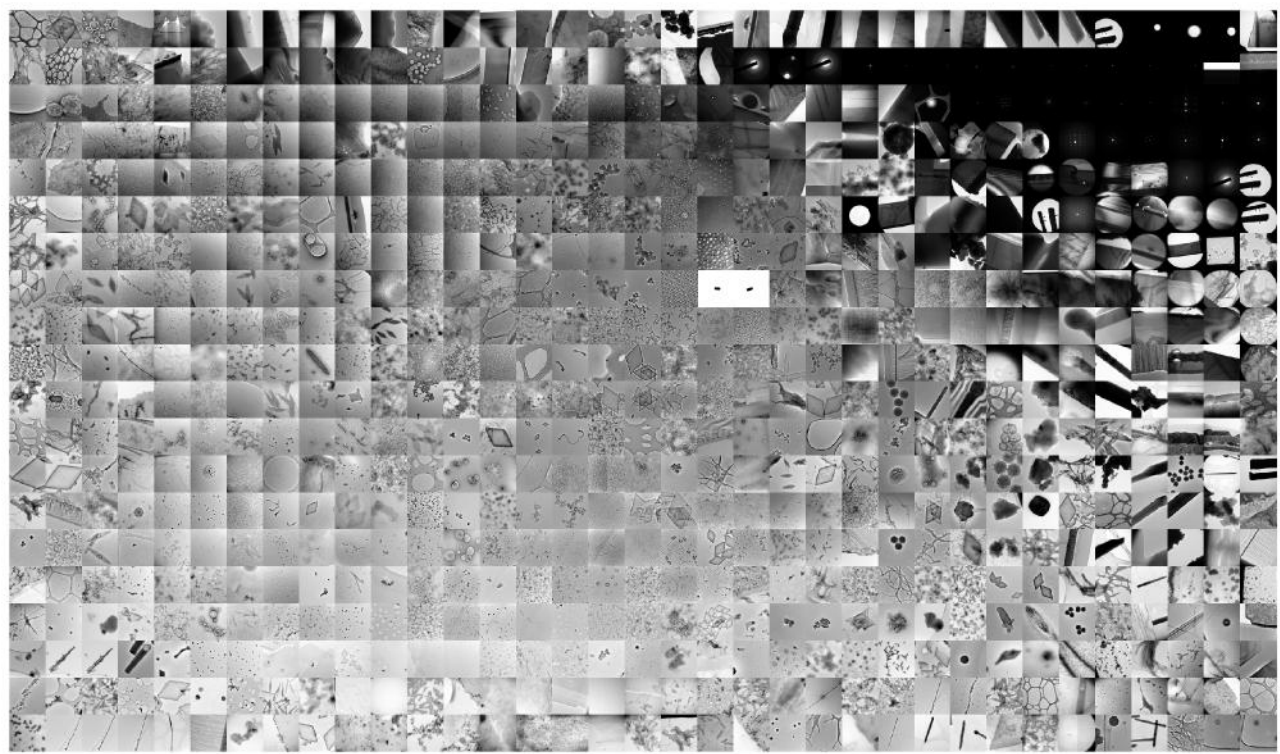

**Figure S13.** Two-dimensional uniformly separated tSNE visualization of 64-dimensional VAE latent spaces for 17266 TEM images that have been downsampled to  $96 \times 96$ .

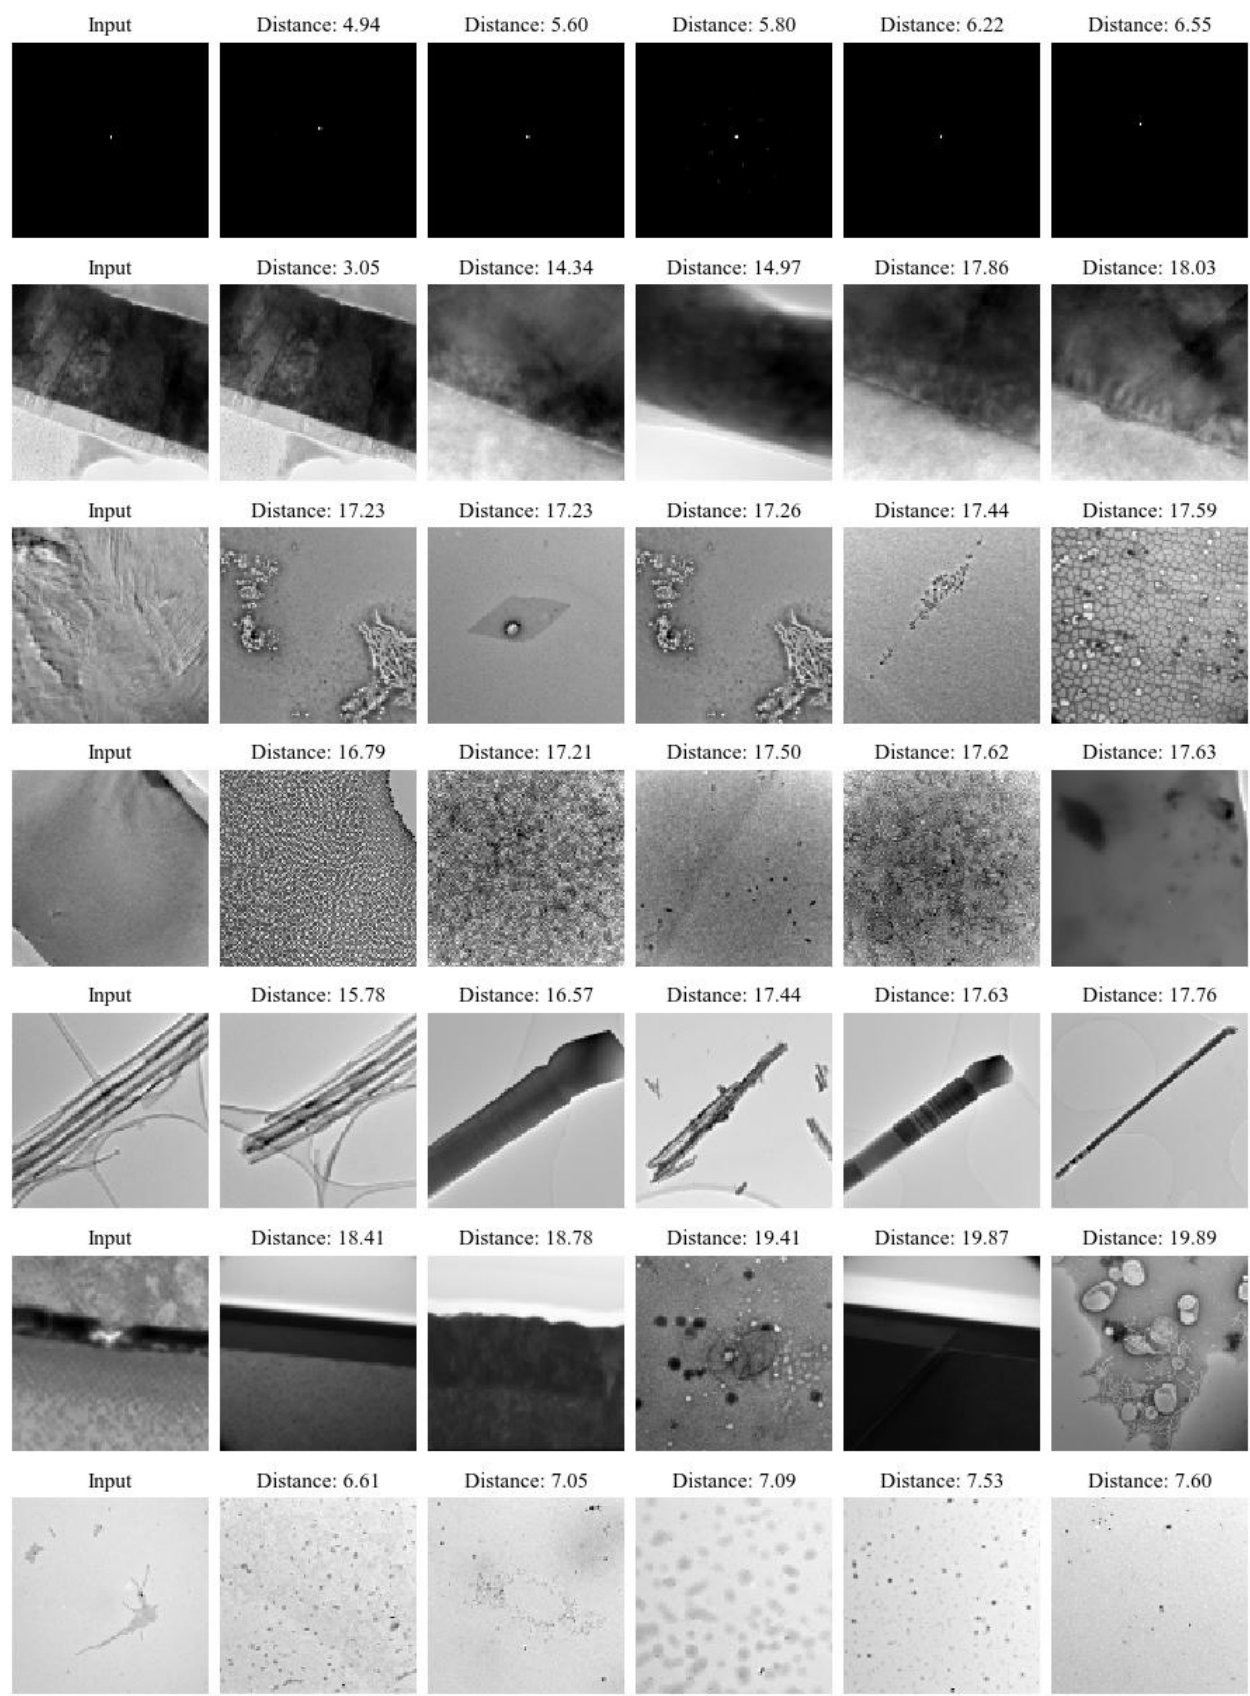

**Figure S14.** Examples of top-5 search results for  $96 \times 96$  TEM images. Euclidean distances between  $\mu$  encoded for search inputs and results are smaller for more similar images.

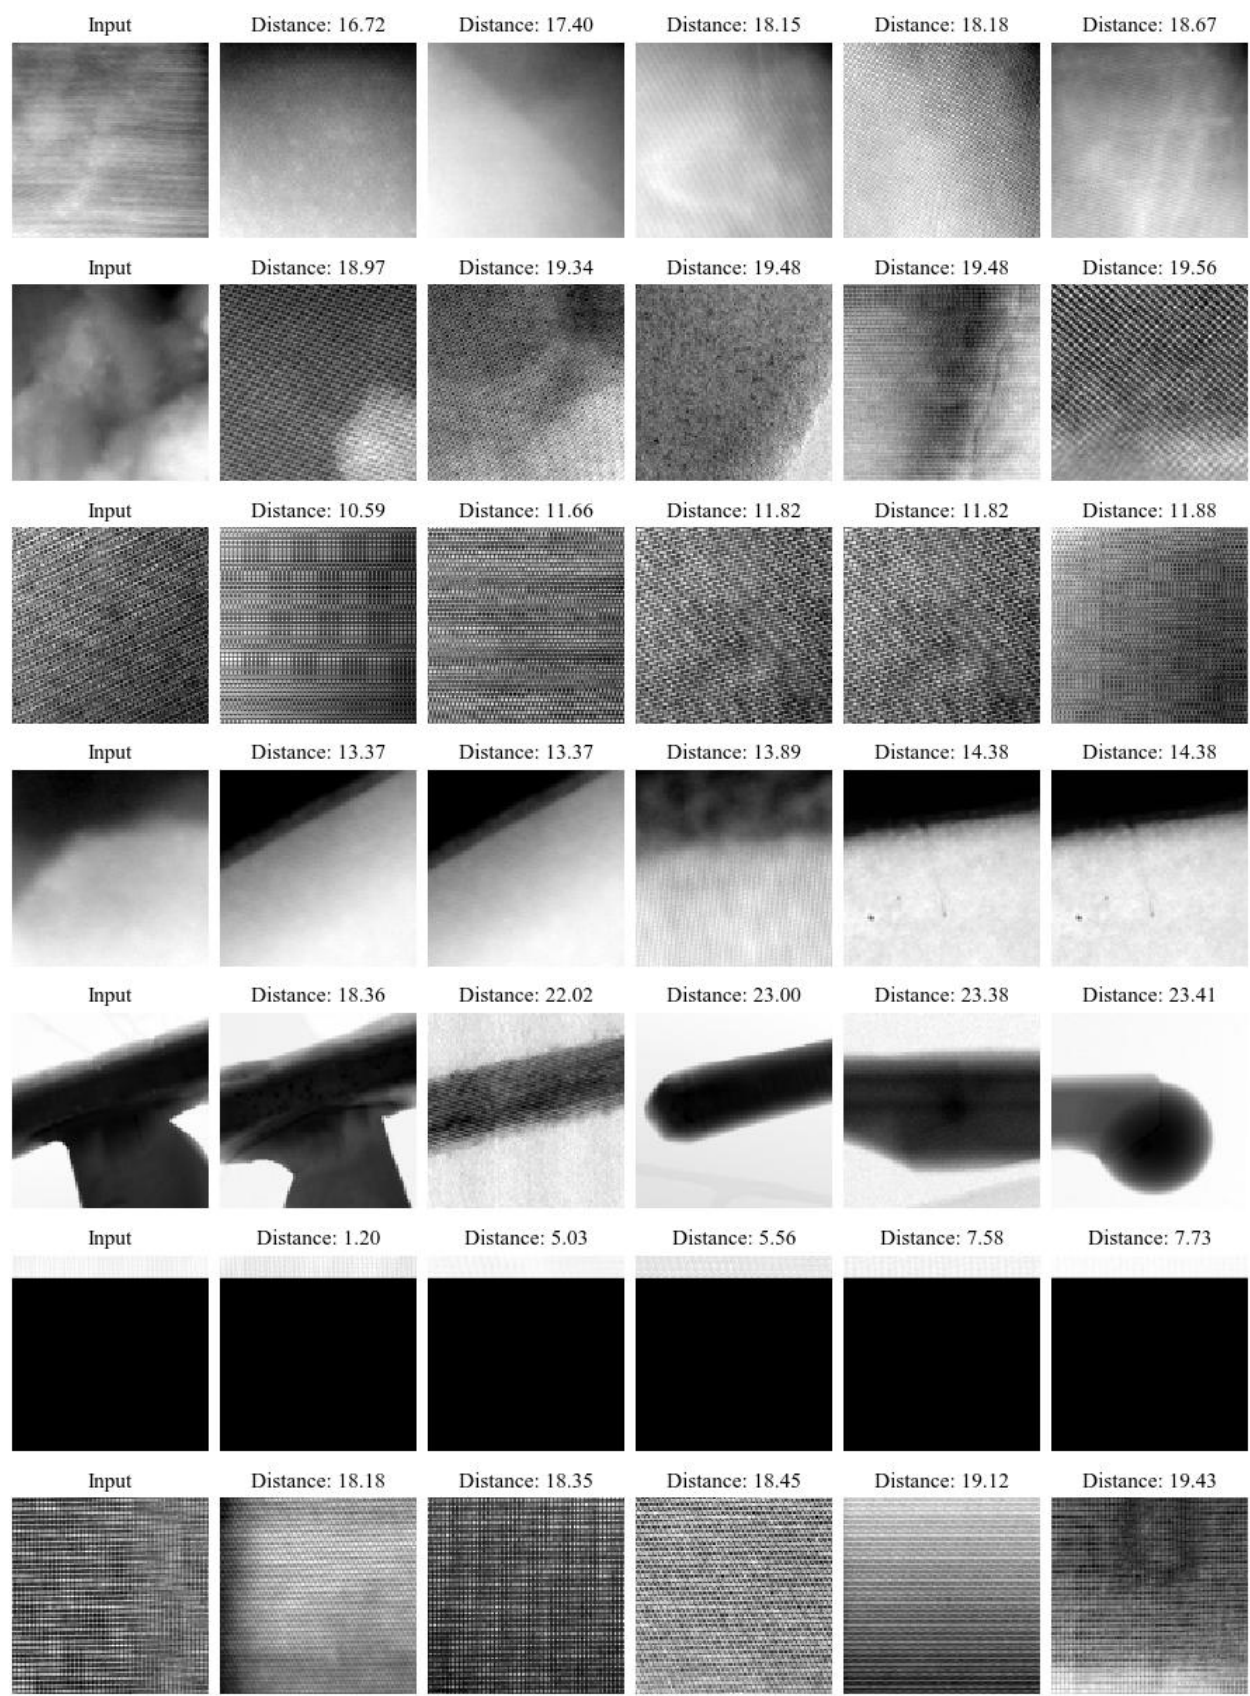

**Figure S15.** Examples of top-5 search results for  $96 \times 96$  STEM images. Euclidean distances between  $\mu$  encoded for search inputs and results are smaller for more similar images.
