# Supplementary material for: Advances in Electron Microscopy with Deep Learning
Source: arXiv:2101.01178 source file (2021-03-11)
Supplement: Supplementary file 4 [file paper_wavefunctions_supplementary.pdf]

# Supplementary Information: Exit Wavefunction Reconstruction from Single Transmission Electron Micrographs with Deep Learning

Jeffrey M. Ede, Jonathan J. P. Peters, Jeremy Sloan, and Richard Beanland

{j.m.ede, j.peters.1, j.sloan, r.beanland}@warwick.ac.uk

## S1. ADDITIONAL EXAMPLES

Example applications of ANNs are shown in figs. S1-S18, and source code for every ANN is available in [1]. Phases in  $[-\pi, \pi)$  rad are depicted on a linear greyscale from black to white. Wavefunctions are cyclically periodic functions of phase so distances between black and white pixels are small.

## REFERENCES

- [1] J. M. Ede, “One shot exit wavefunction reconstruction.” online: <https://github.com/Jeffrey-Ede/one-shot>, 2019.

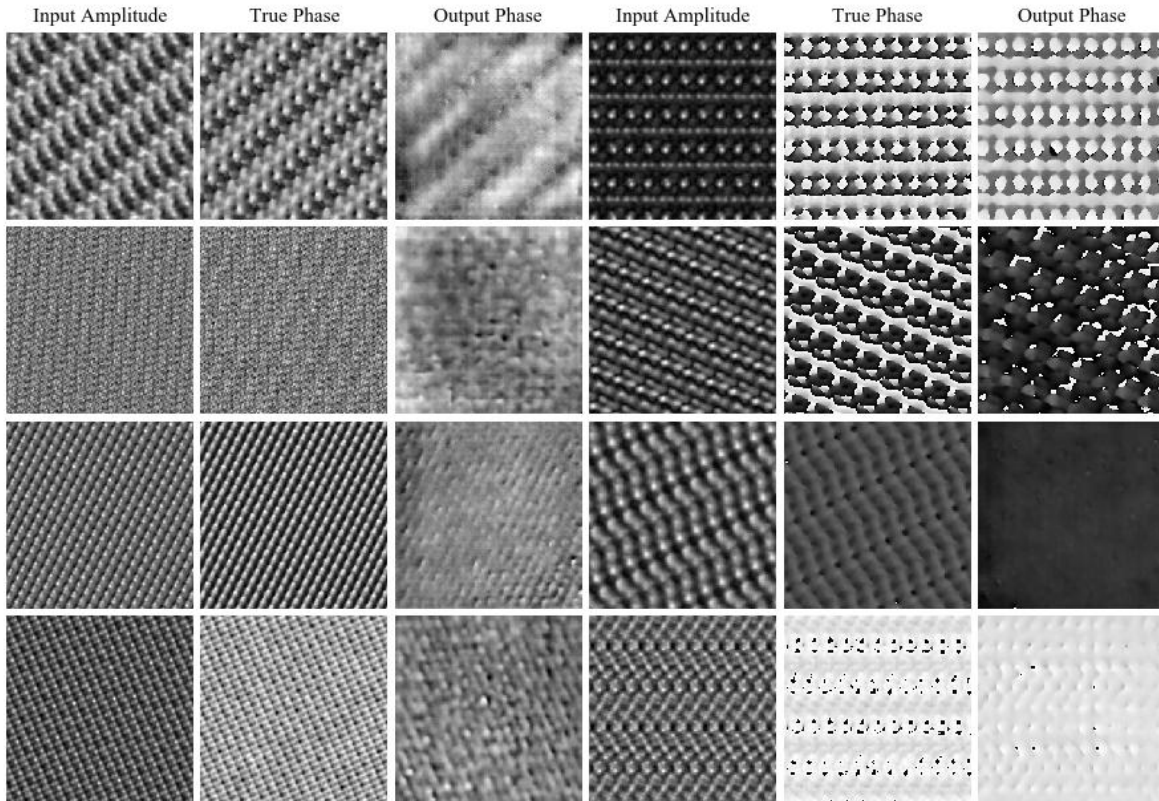

**Fig. S1:** Input amplitudes, target phases and output phases of  $224 \times 224$  multiple material training set wavefunctions for unseen flips, rotations and translations, and  $n = 1$  simulation physics.

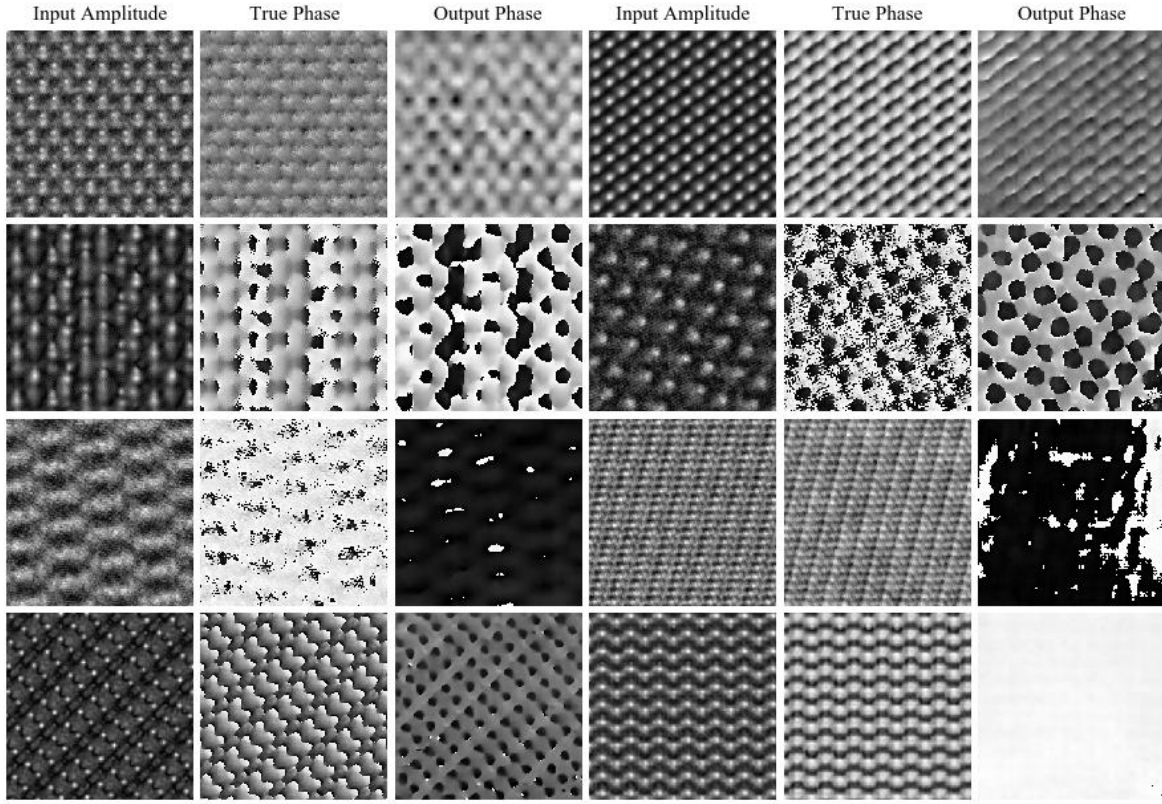

**Fig. S2:** Input amplitudes, target phases and output phases of  $224 \times 224$  multiple material validation set wavefunctions for seen materials, unseen simulation hyperparameters, and  $n = 1$  simulation physics.

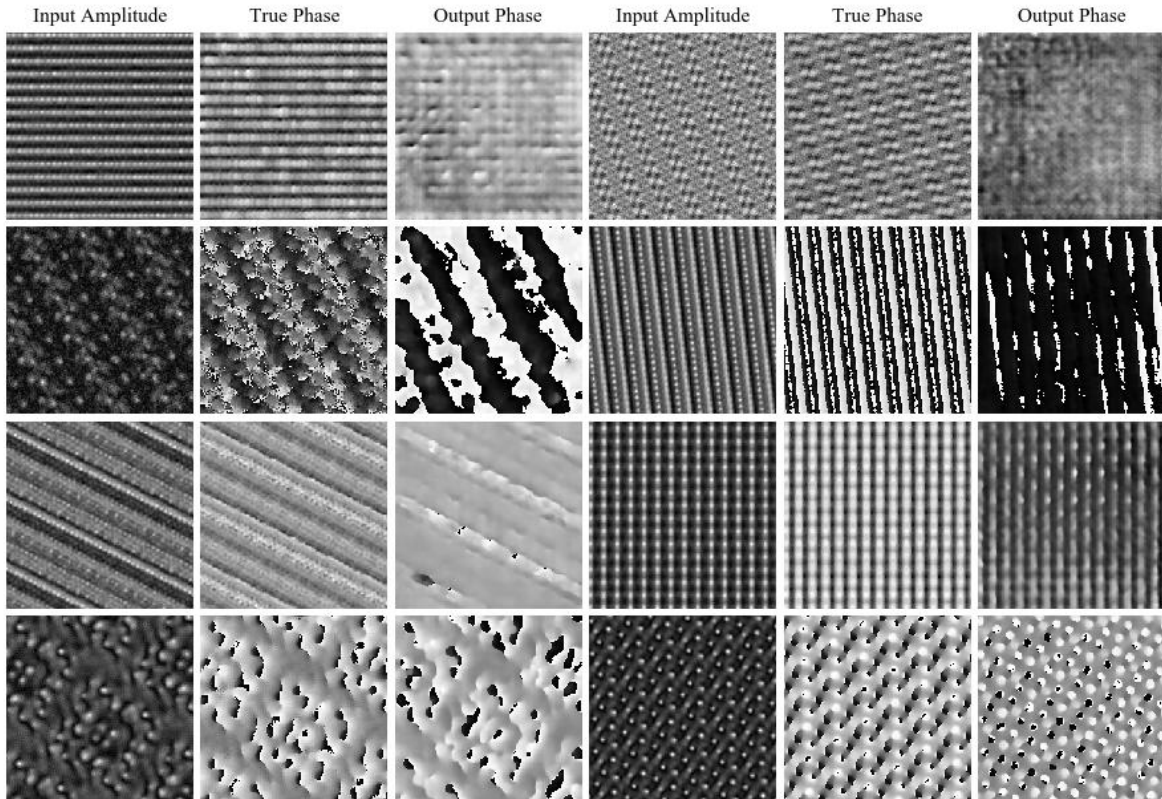

**Fig. S3:** Input amplitudes, target phases and output phases of  $224 \times 224$  multiple material validation set wavefunctions for unseen materials, unseen simulation hyperparameters, and  $n = 1$  simulation physics.

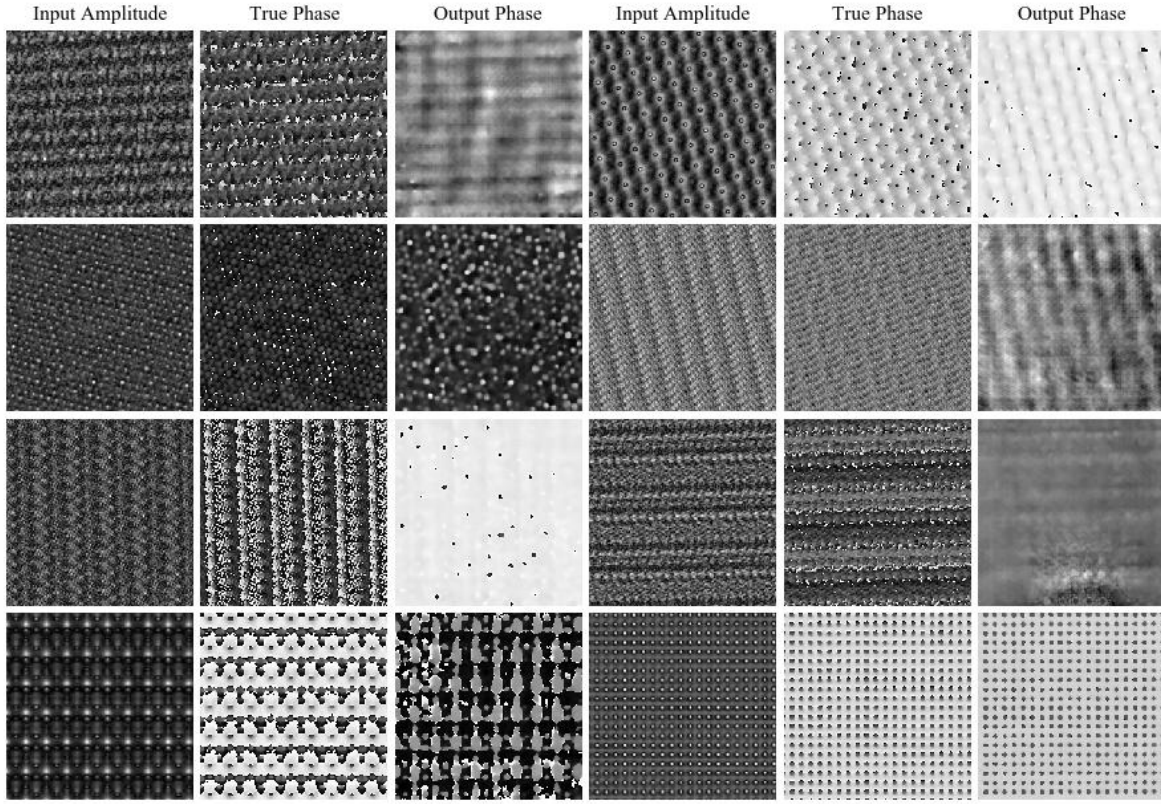

**Fig. S4:** Input amplitudes, target phases and output phases of  $224 \times 224$  multiple material training set wavefunctions for unseen flips, rotations and translations, and  $n = 3$  simulation physics.

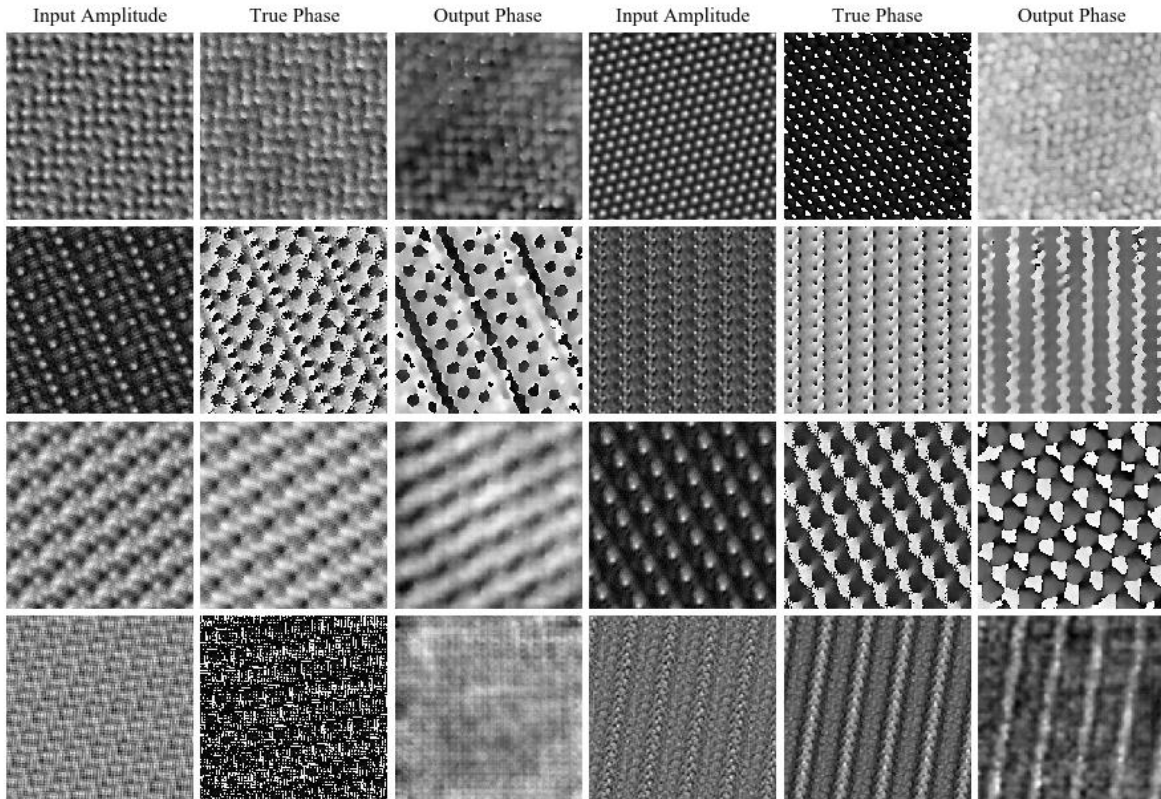

**Fig. S5:** Input amplitudes, target phases and output phases of  $224 \times 224$  multiple material validation set wavefunctions for seen materials, unseen simulation hyperparameters, and  $n = 3$  simulation physics.



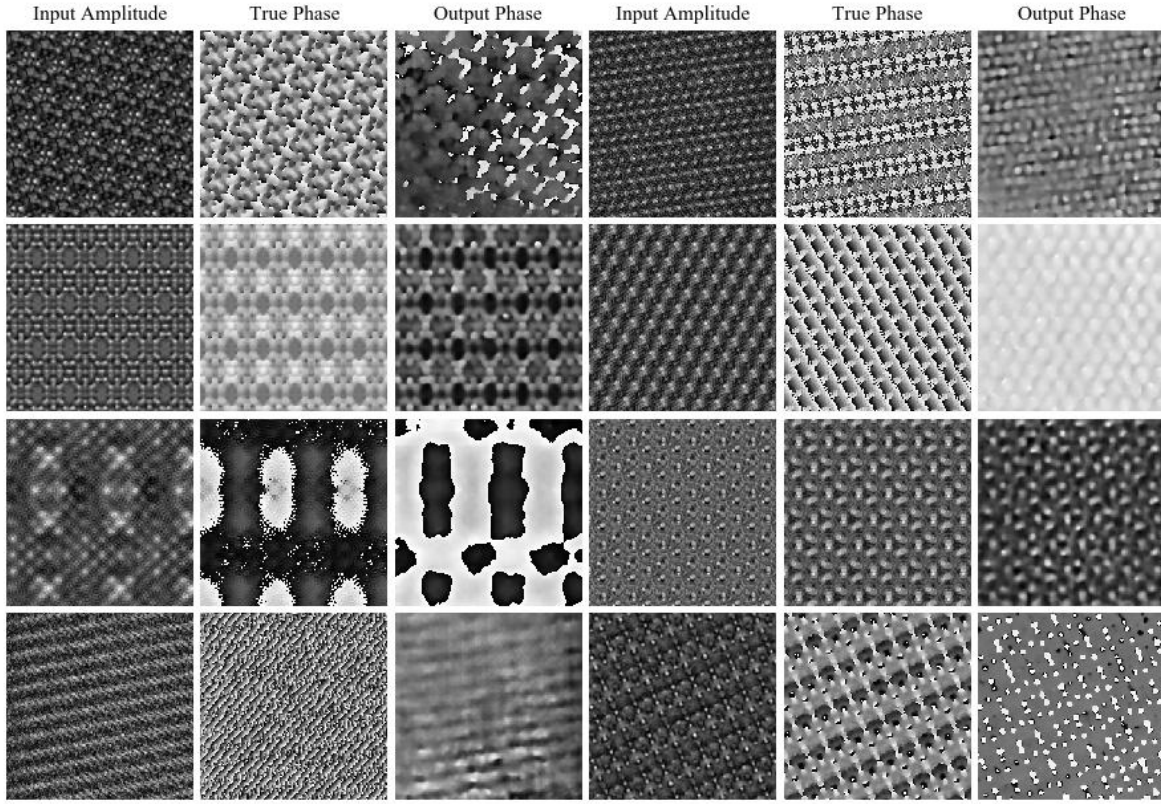

**Fig. S6:** Input amplitudes, target phases and output phases of  $224 \times 224$  multiple material validation set wavefunctions for unseen materials, unseen simulation hyperparameters are unseen, and  $n = 3$  simulation physics.

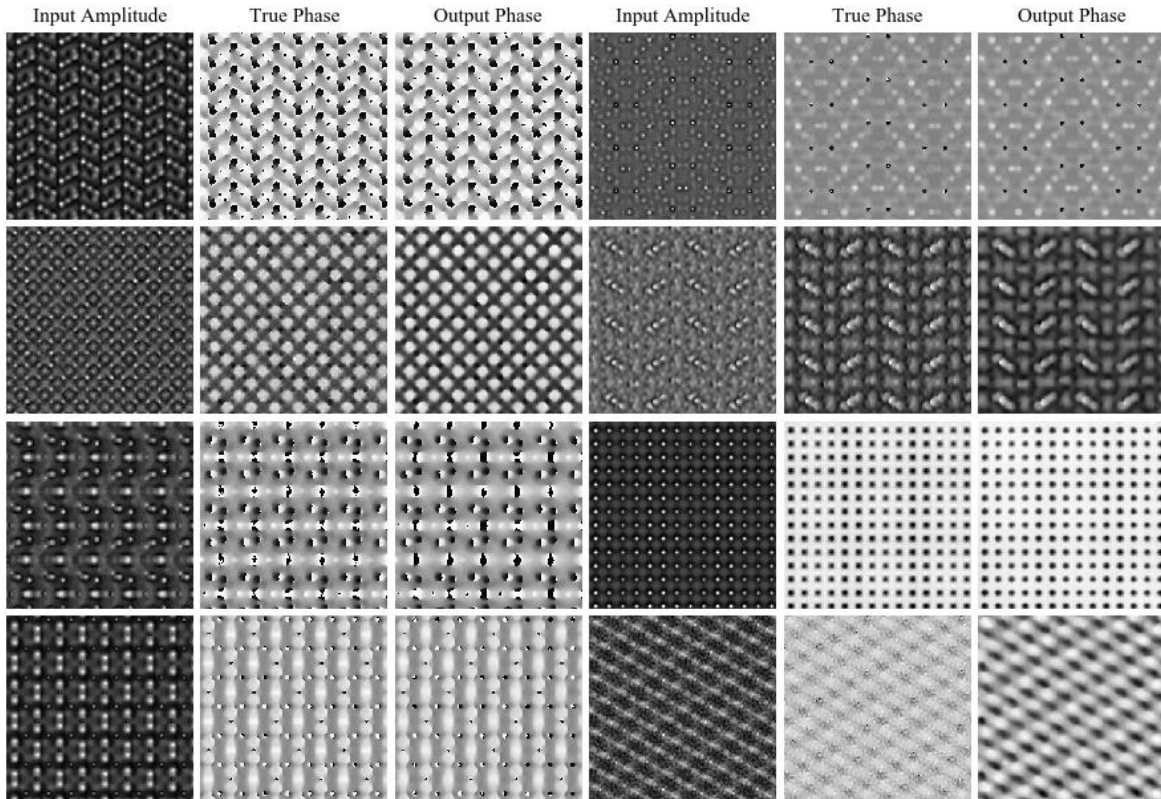

**Fig. S7:** Input amplitudes, target phases and output phases of  $224 \times 224$  validation set wavefunctions for restricted simulation hyperparameters, and  $n = 3$  simulation physics.

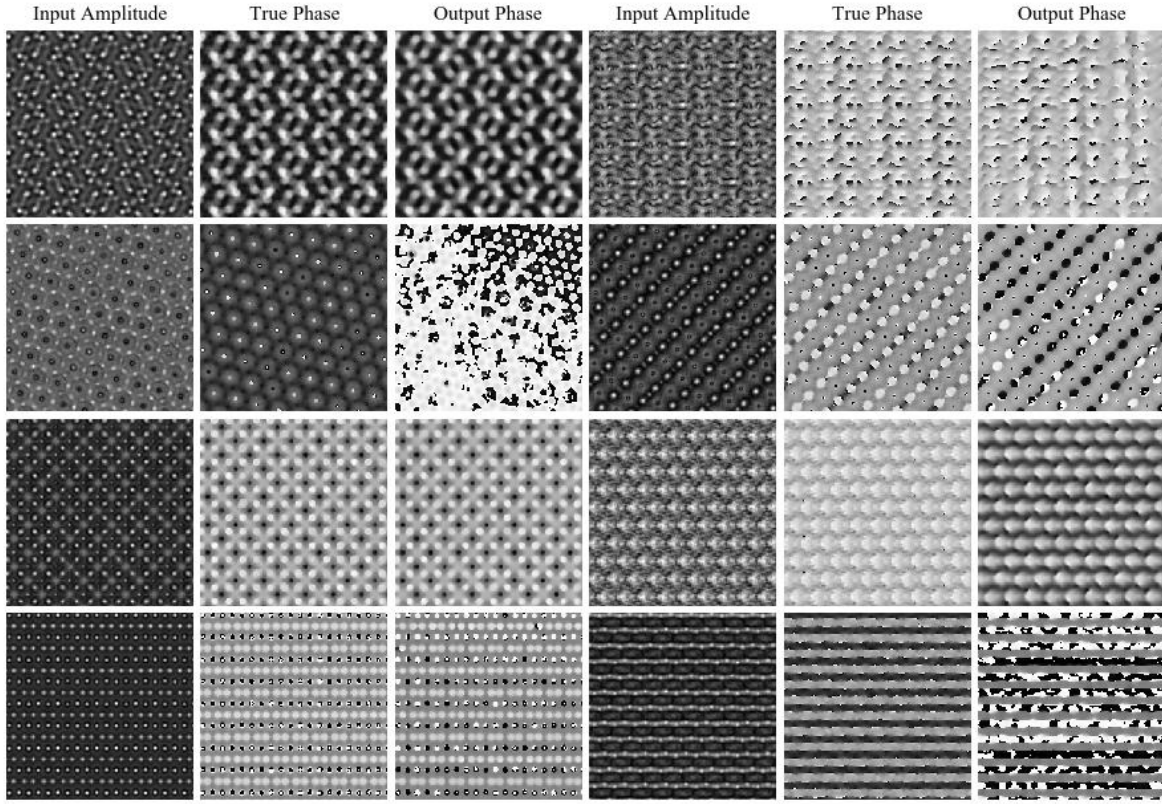

**Fig. S8:** Input amplitudes, target phases and output phases of  $224 \times 224$  validation set wavefunctions for restricted simulation hyperparameters, and  $n = 3$  simulation physics.

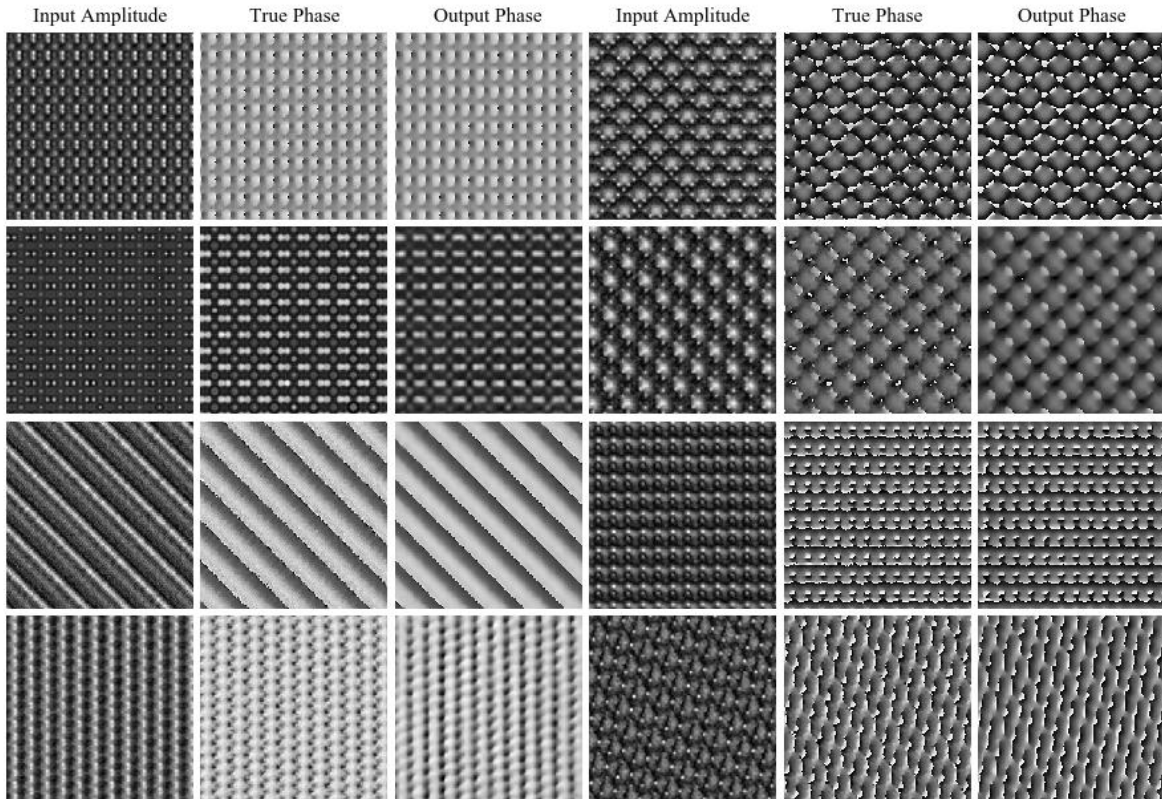

**Fig. S9:** Input amplitudes, target phases and output phases of  $224 \times 224$   $\text{In}_{1.7}\text{K}_2\text{Se}_8\text{Sn}_{2.28}$  training set wavefunctions for unseen flips, rotations and translations, and  $n = 1$  simulation physics.

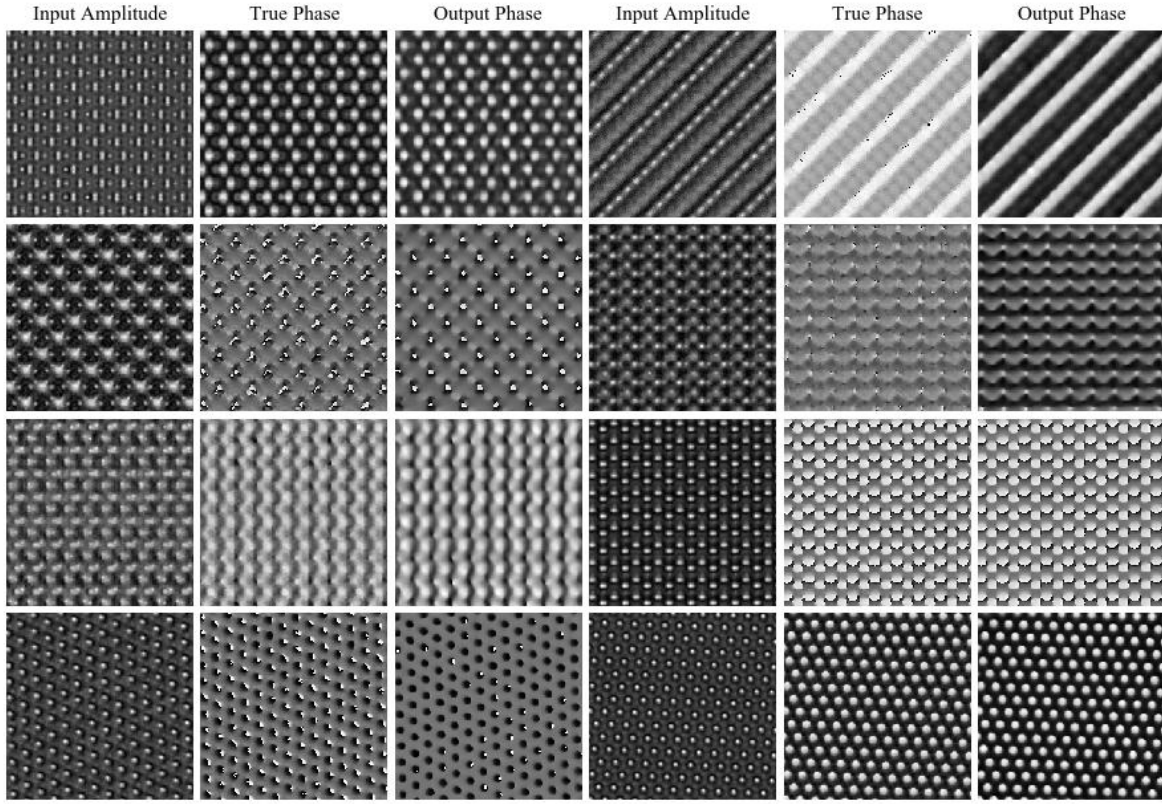

**Fig. S10:** Input amplitudes, target phases and output phases of  $224 \times 224$   $\text{In}_{1.7}\text{K}_2\text{Se}_8\text{Sn}_{2.28}$  validation set wavefunctions for unseen simulation hyperparameters, and  $n = 1$  simulation physics.

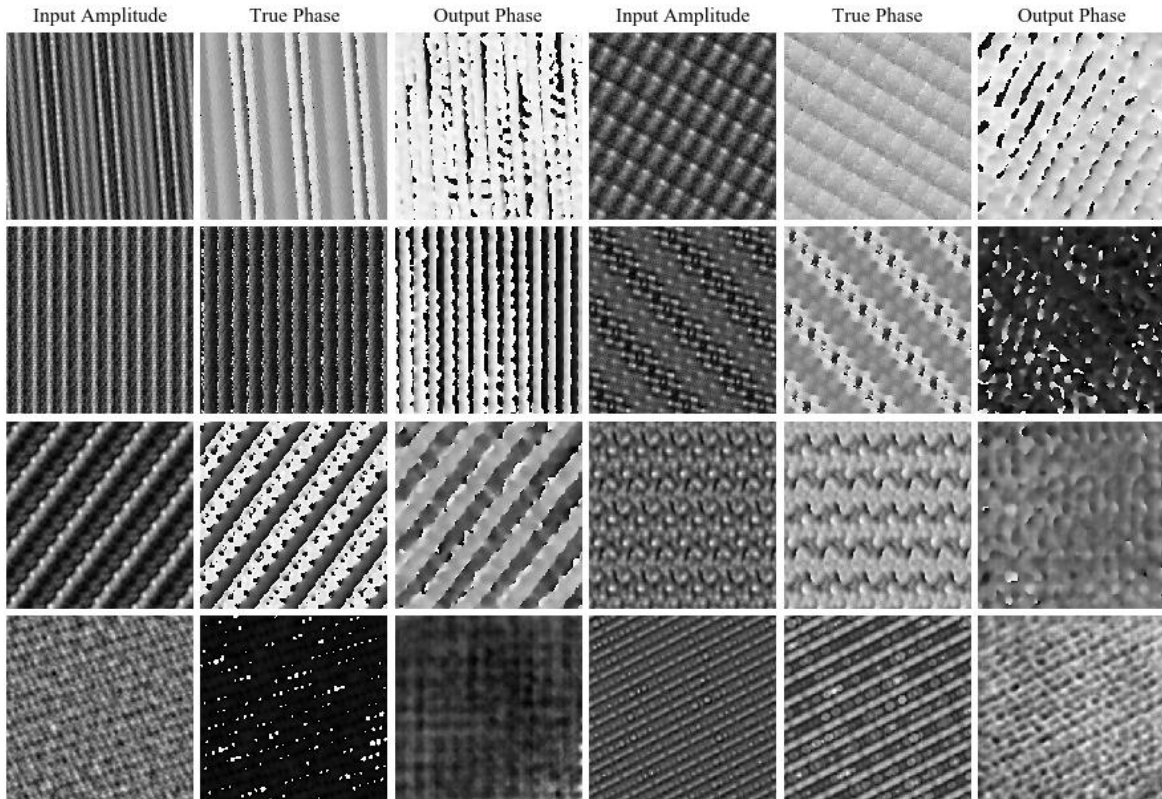

**Fig. S11:** Input amplitudes, target phases and output phases of  $224 \times 224$  validation set wavefunctions for unseen simulation hyperparameters and materials, and  $n = 1$  simulation physics. The generator was trained with  $\text{In}_{1.7}\text{K}_2\text{Se}_8\text{Sn}_{2.28}$  wavefunctions.



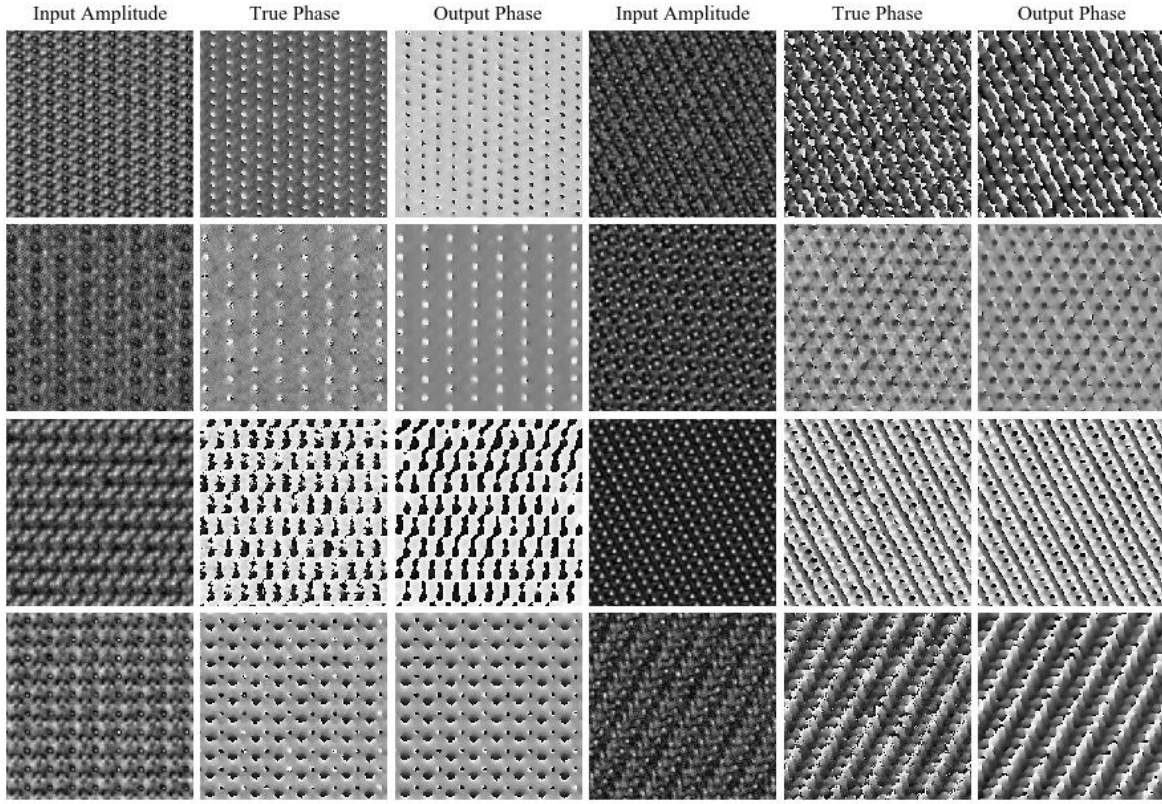

**Fig. S12:** Input amplitudes, target phases and output phases of  $224 \times 224$   $\text{In}_{1.7}\text{K}_2\text{Se}_8\text{Sn}_{2.28}$  training set wavefunctions for unseen flips, rotations and translations, and  $n = 1$  simulation physics.

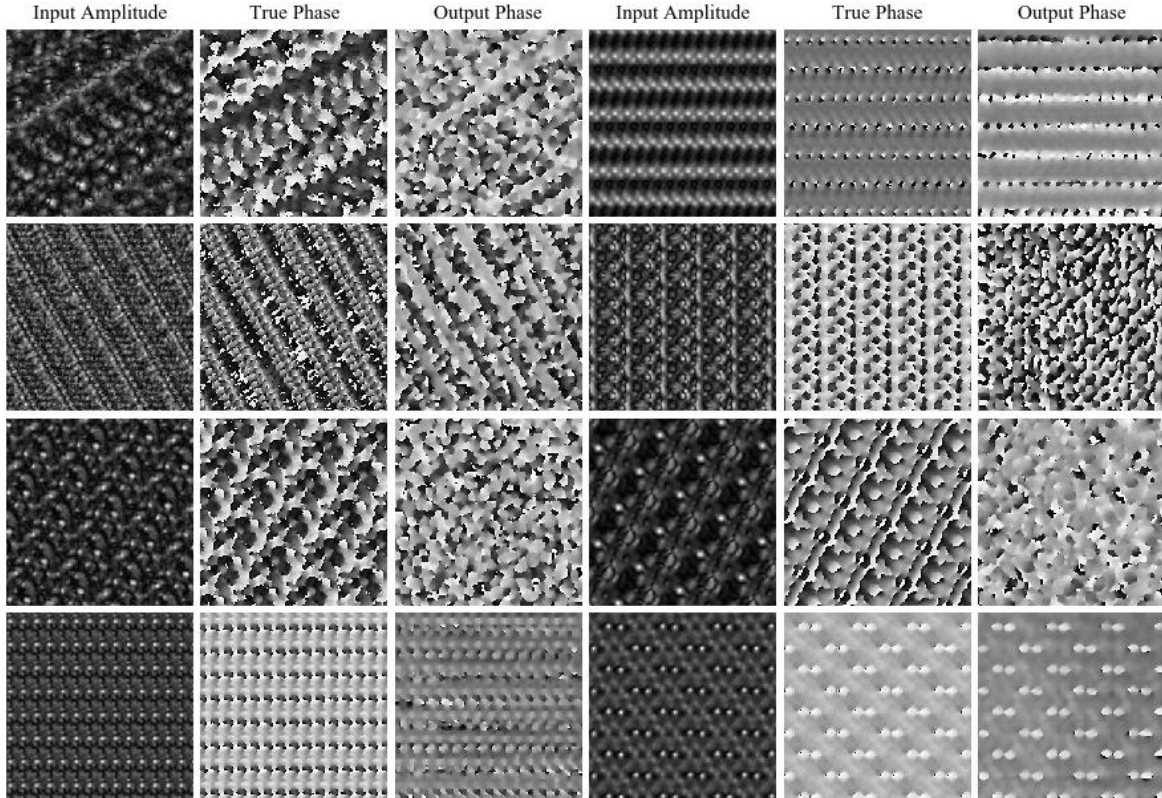

**Fig. S13:** Input amplitudes, target phases and output phases of  $224 \times 224$   $\text{In}_{1.7}\text{K}_2\text{Se}_8\text{Sn}_{2.28}$  validation set wavefunctions for unseen simulation hyperparameters, and  $n = 3$  simulation physics.

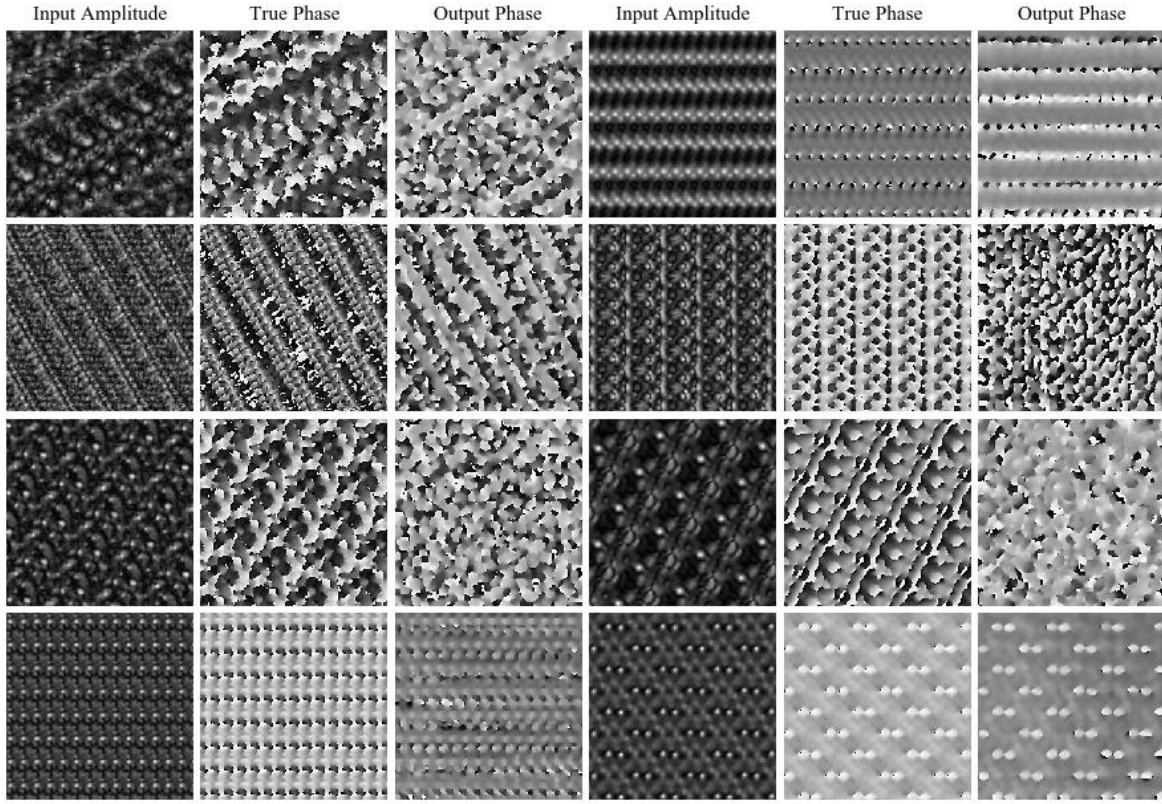

**Fig. S14:** Input amplitudes, target phases and output phases of  $224 \times 224$  validation set wavefunctions for unseen simulation hyperparameters and materials, and  $n = 3$  simulation physics. The generator was trained with  $\text{In}_{1.7}\text{K}_2\text{Se}_8\text{Sn}_{2.28}$  wavefunctions.

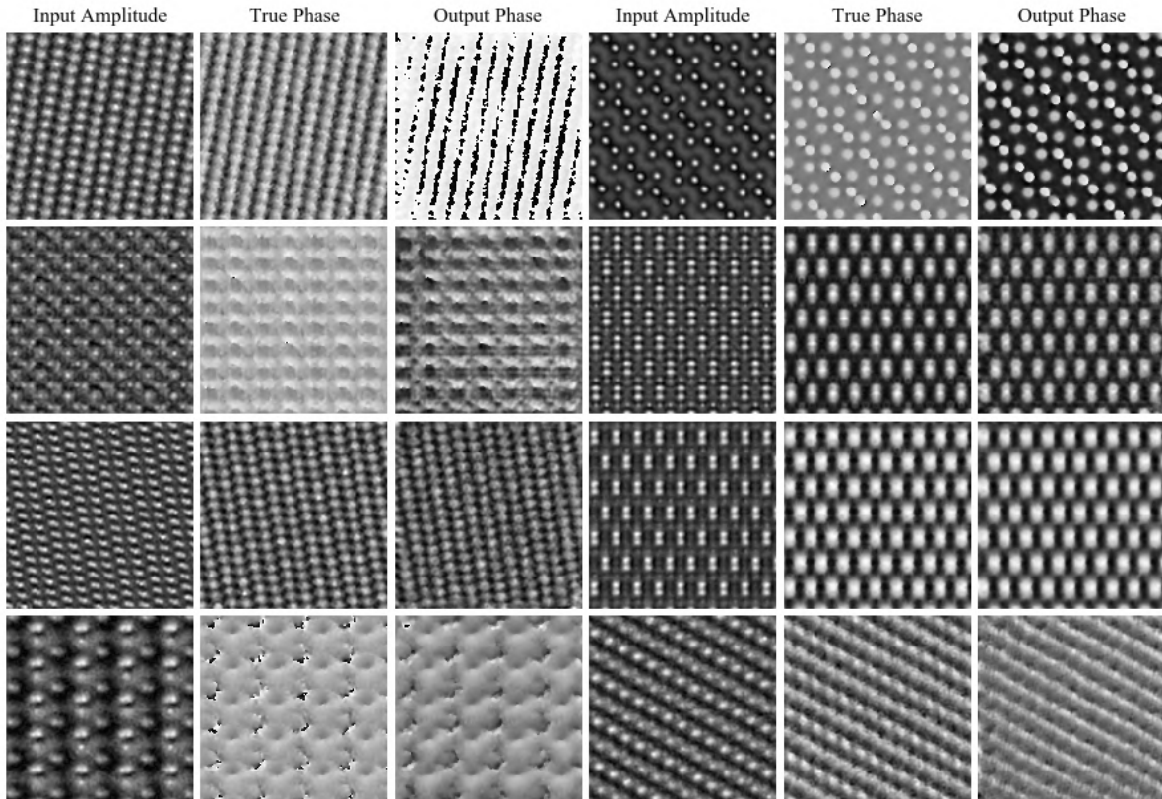

**Fig. S15:** GAN input amplitudes, target phases and output phases of  $144 \times 144$   $\text{In}_{1.7}\text{K}_2\text{Se}_8\text{Sn}_{2.28}$  validation set wavefunctions for unseen flips, rotations and translations, and  $n = 1$  simulation physics.



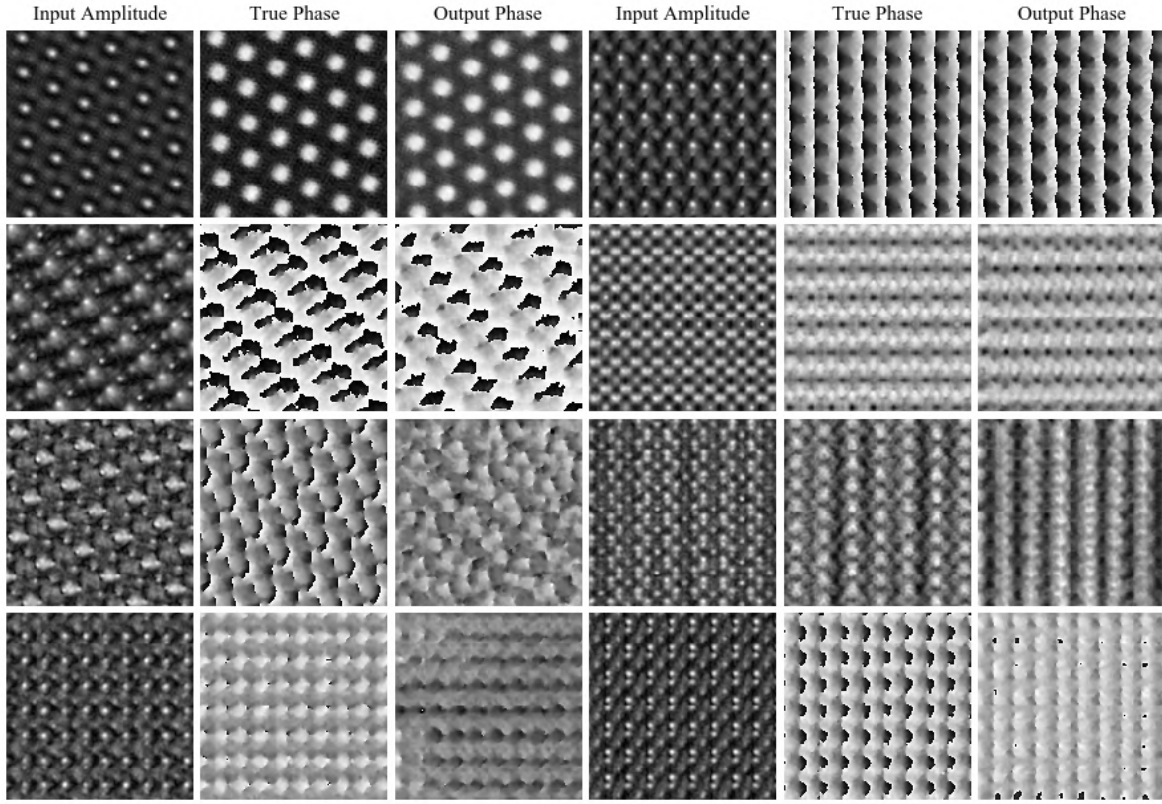

**Fig. S16:** GAN input amplitudes, target phases and output phases of  $144 \times 144$   $\text{In}_{1.7}\text{K}_2\text{Se}_8\text{Sn}_{2.28}$  validation set wavefunctions for unseen simulation hyperparameters, and  $n = 1$  simulation physics.

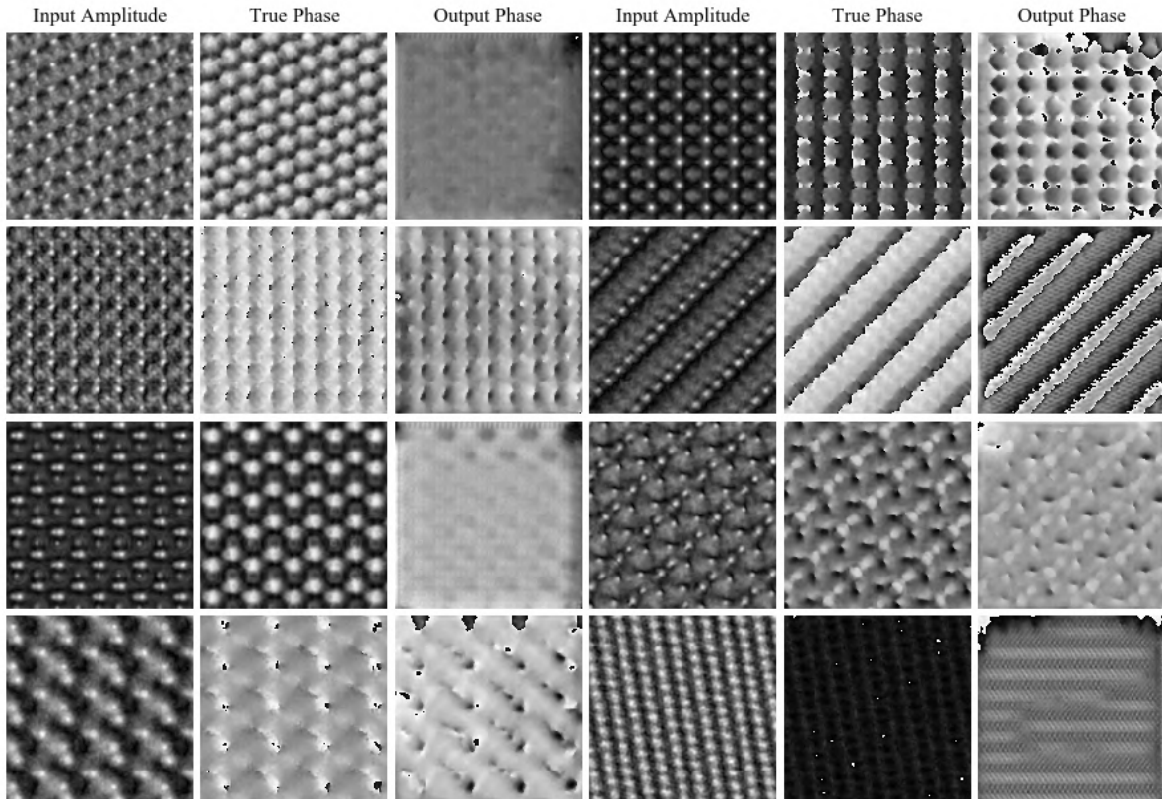

**Fig. S17:** GAN input amplitudes, target phases and output phases of  $144 \times 144$   $\text{In}_{1.7}\text{K}_2\text{Se}_8\text{Sn}_{2.28}$  validation set wavefunctions for unseen flips, rotations and translations, and  $n = 3$  simulation physics.

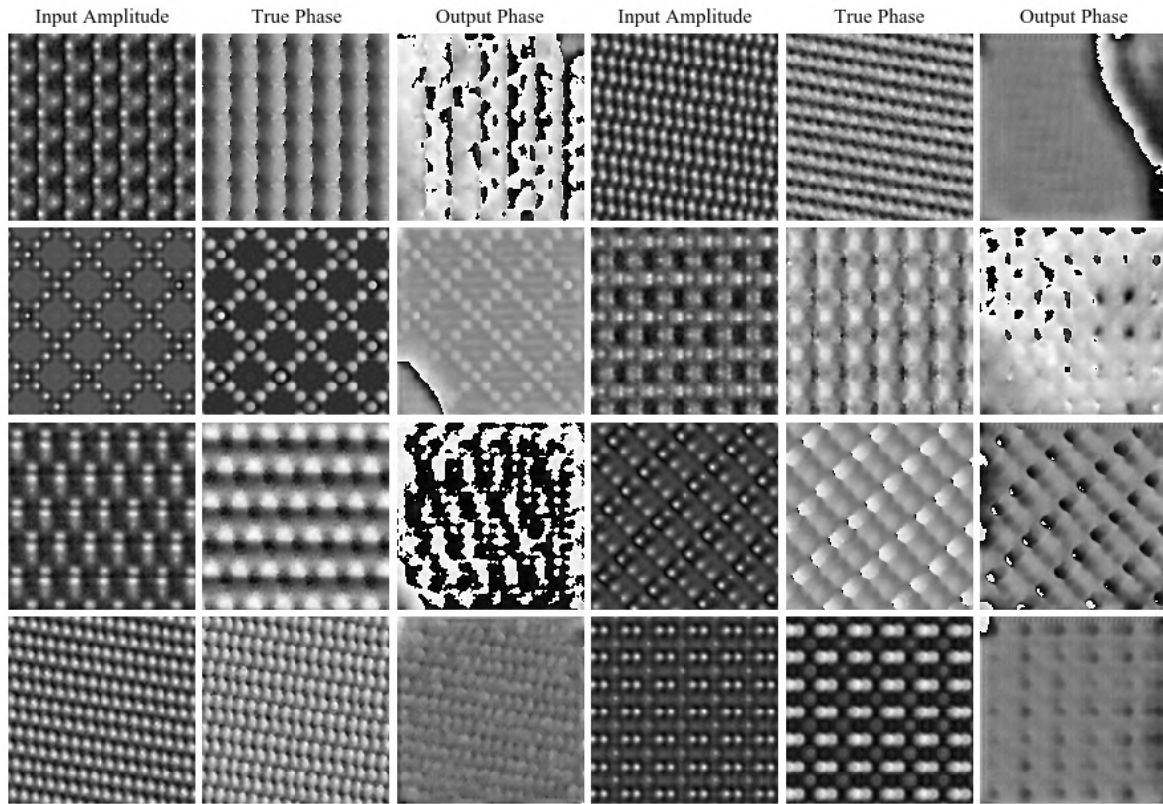

**Fig. S18:** GAN input amplitudes, target phases and output phases of  $144 \times 144$   $\text{In}_{1.7}\text{K}_2\text{Se}_8\text{Sn}_{2.28}$  validation set wavefunctions for unseen simulation hyperparameters, and  $n = 3$  simulation physics.
